# Supplementary material for: Investigating time variability of X-ray absorption in Swift GRBs
Source: arXiv:2301.09292 source file (2023-01-23)

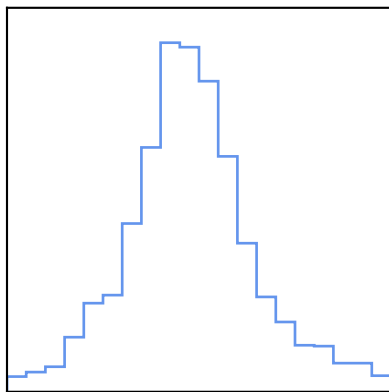

GRB070306

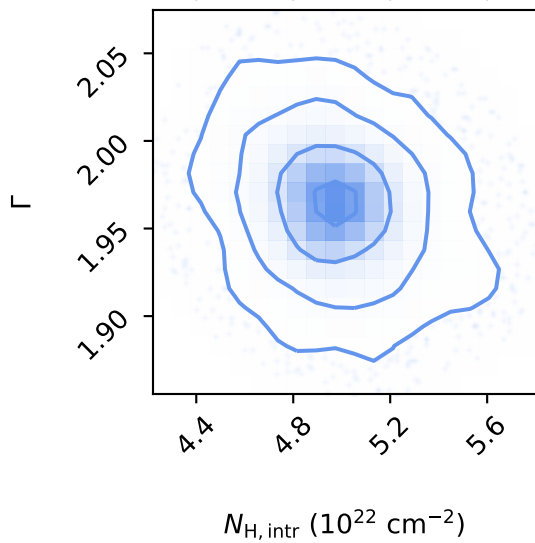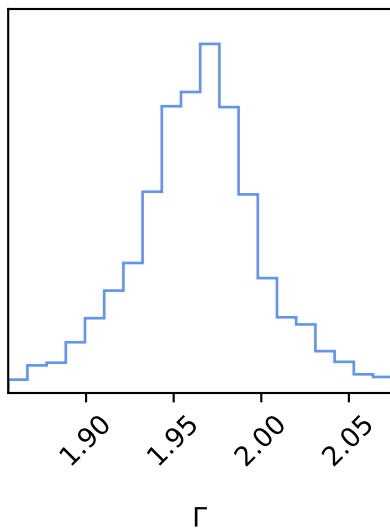

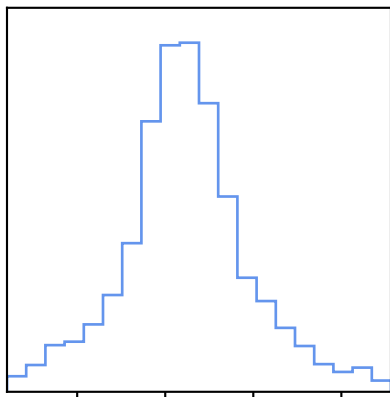

GRB070306

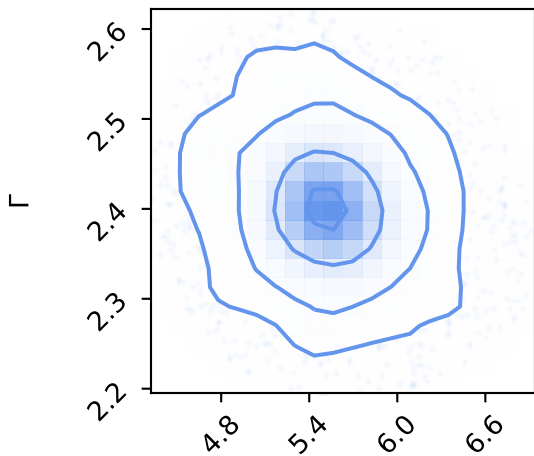

$N_{\text{H,intr}} (10^{22} \text{ cm}^{-2})$

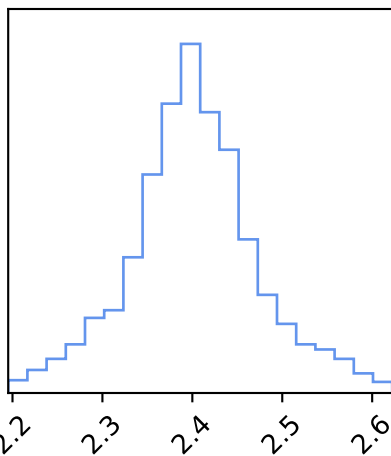

$\Gamma$

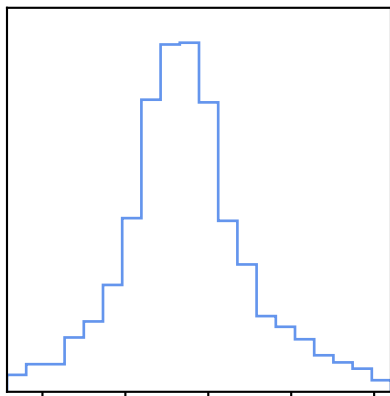

GRB070306

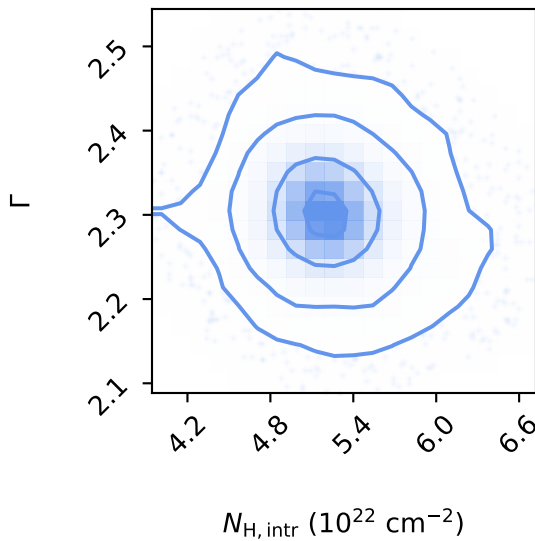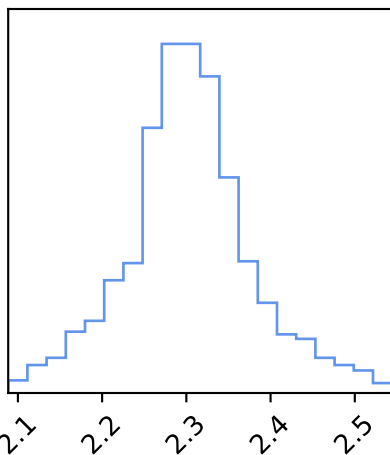

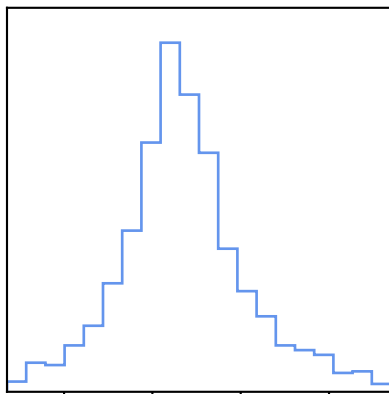

GRB070306

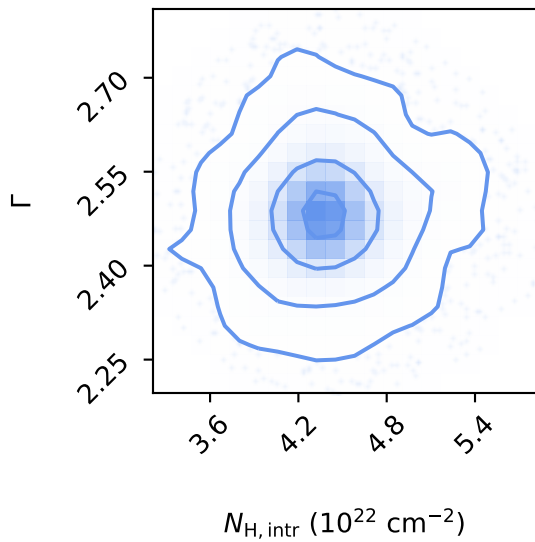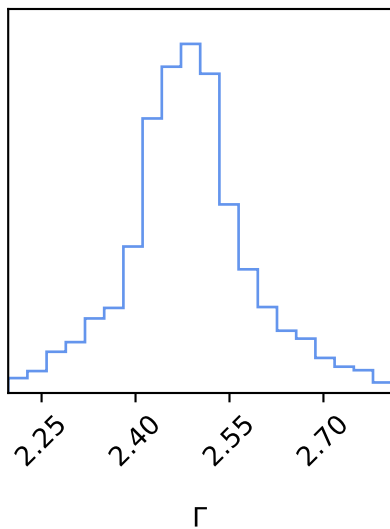

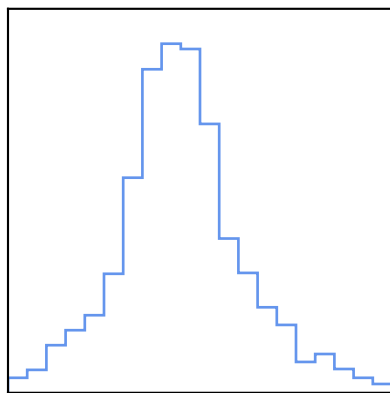

GRB070306

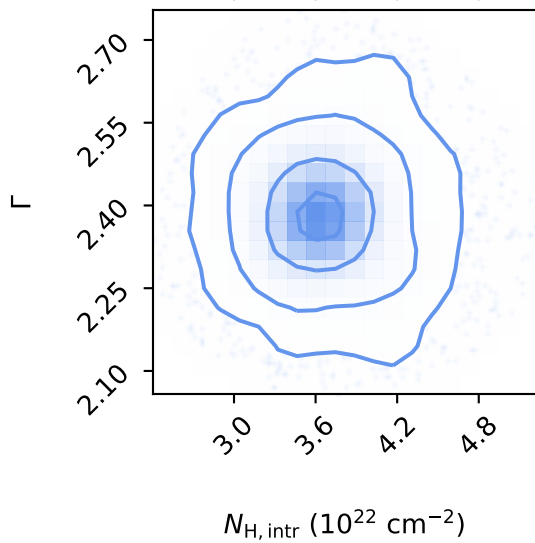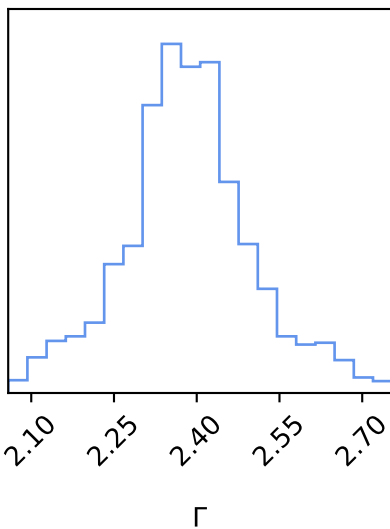

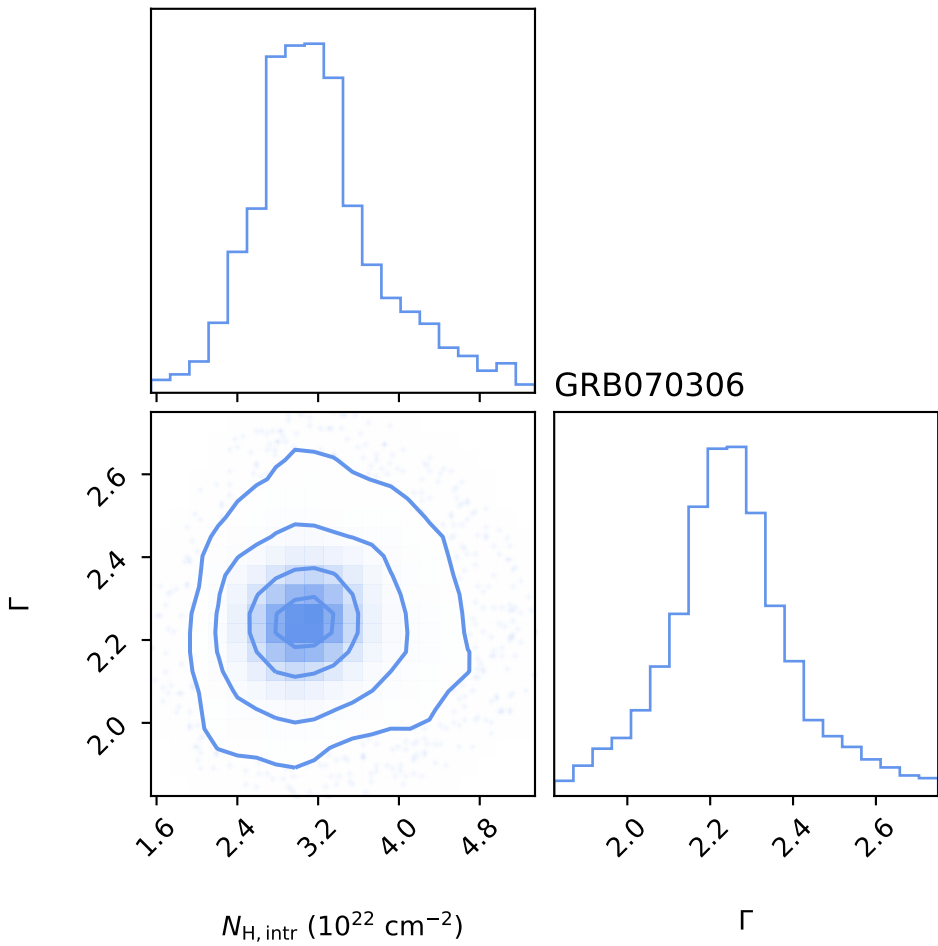

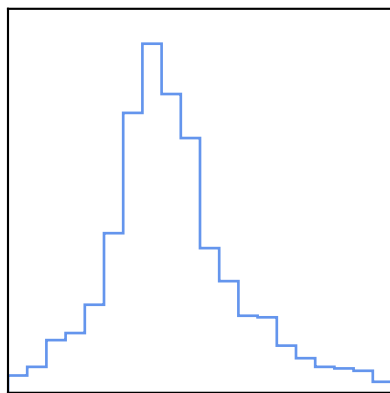

GRB070306

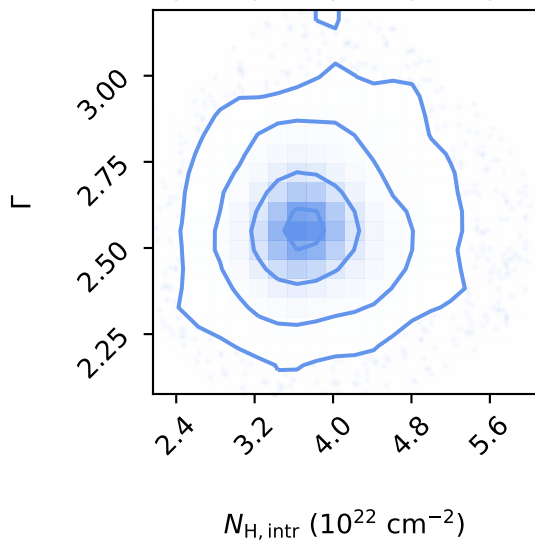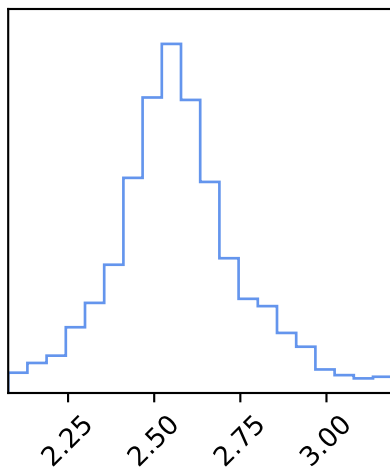

Supplement: Supplementary file 1 [file GRB070306_cornerplot.pdf]
