# Supplementary material for: Investigating time variability of X-ray absorption in Swift GRBs
Source: arXiv:2301.09292 source file (2023-01-23)

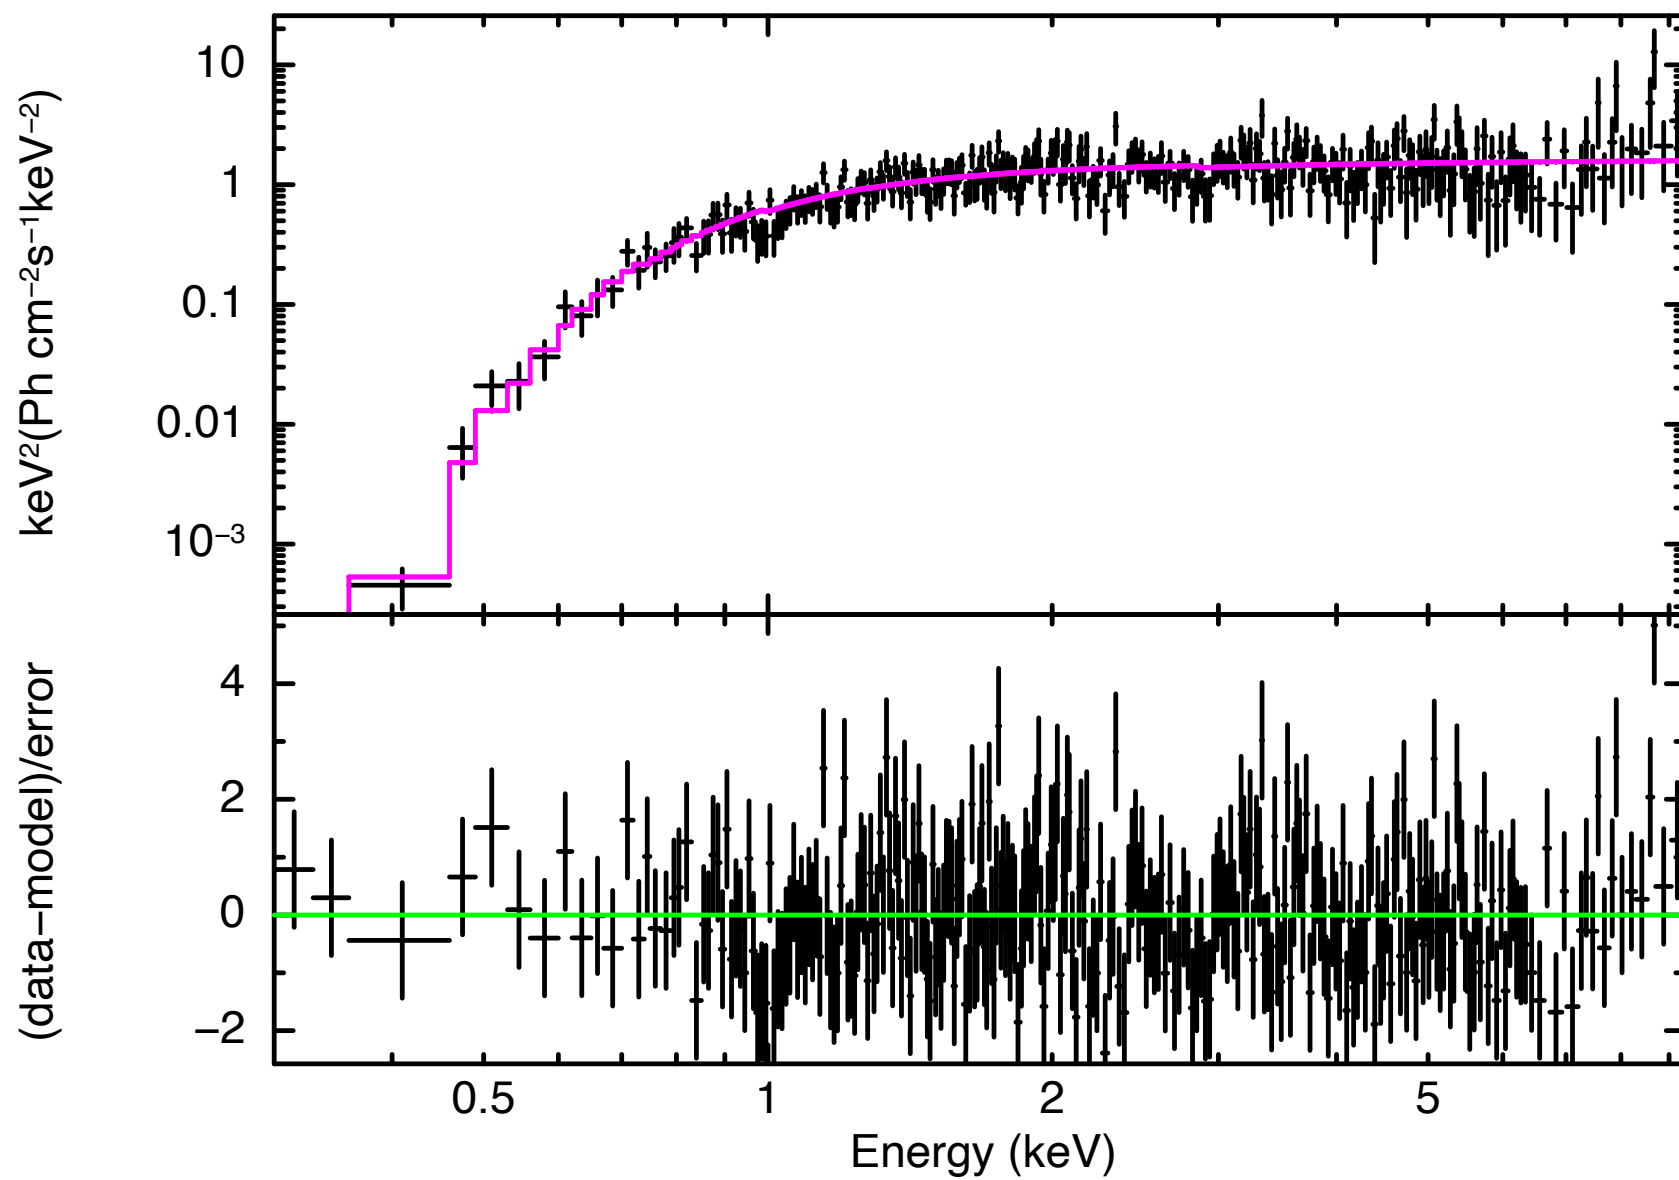

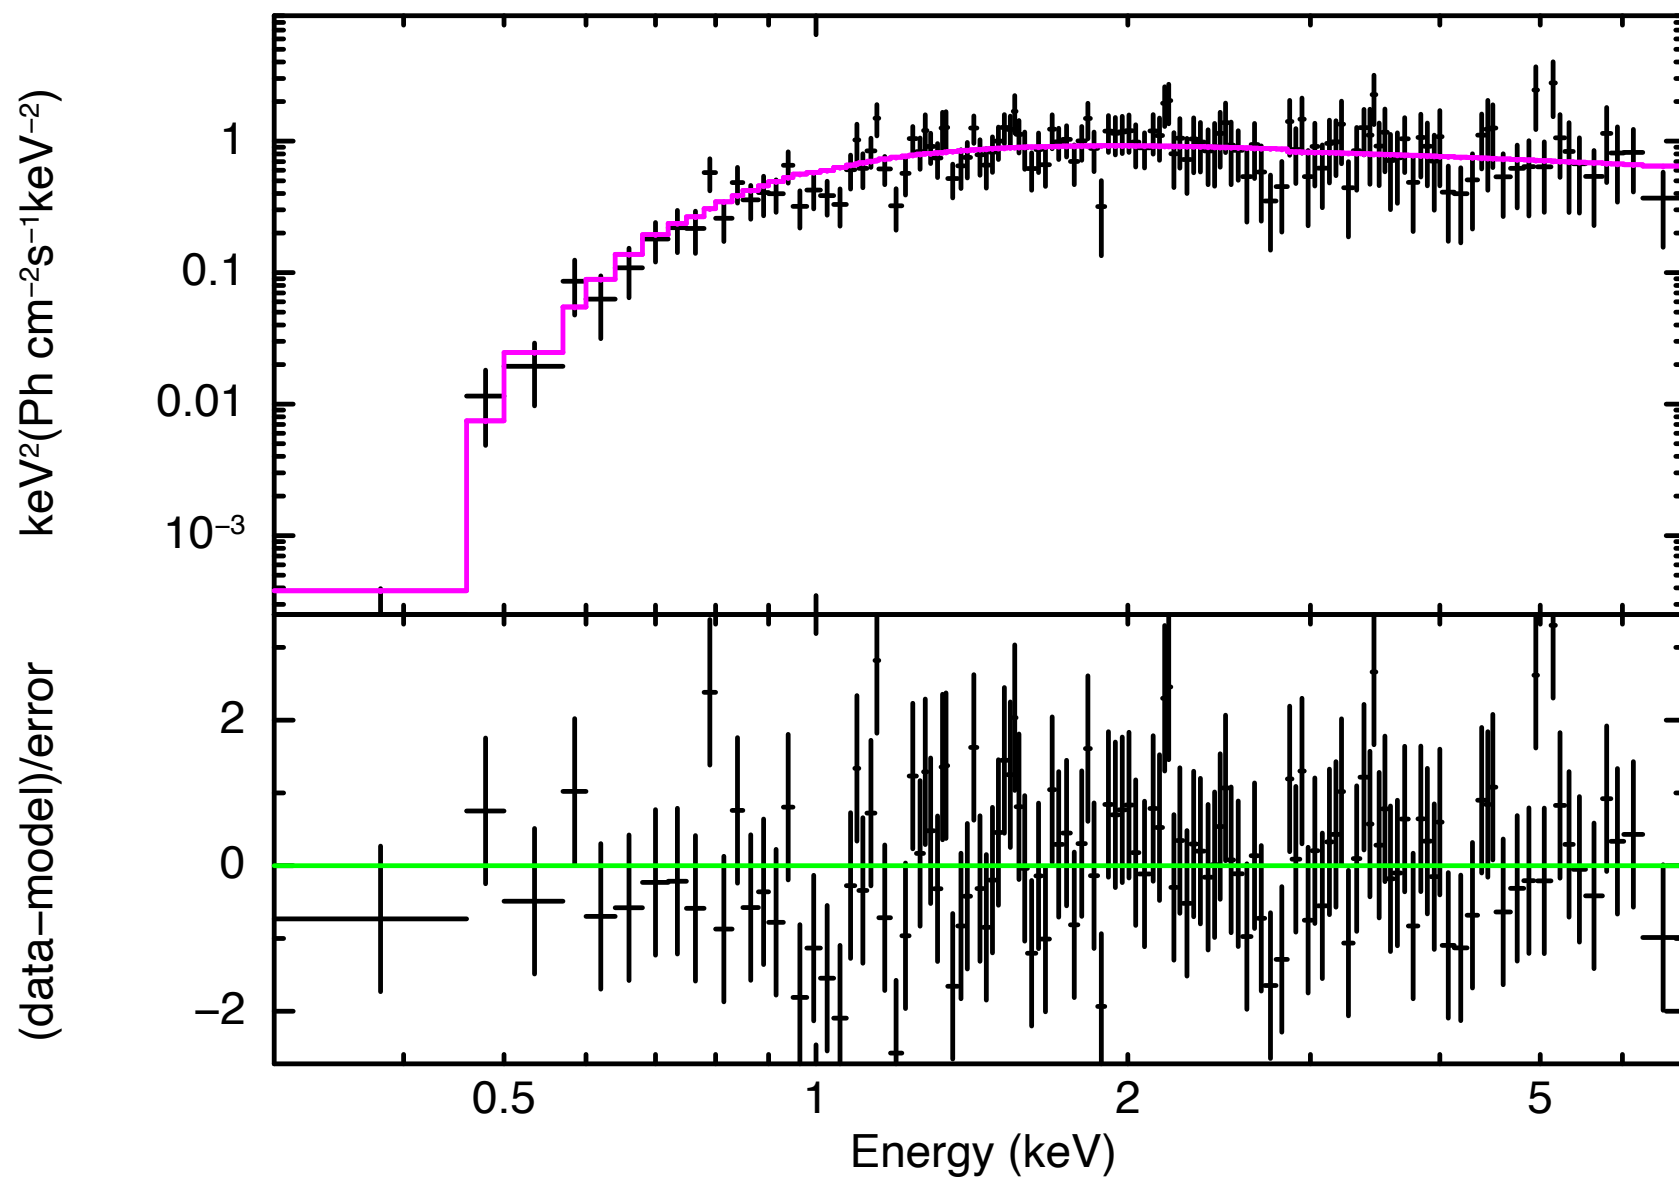

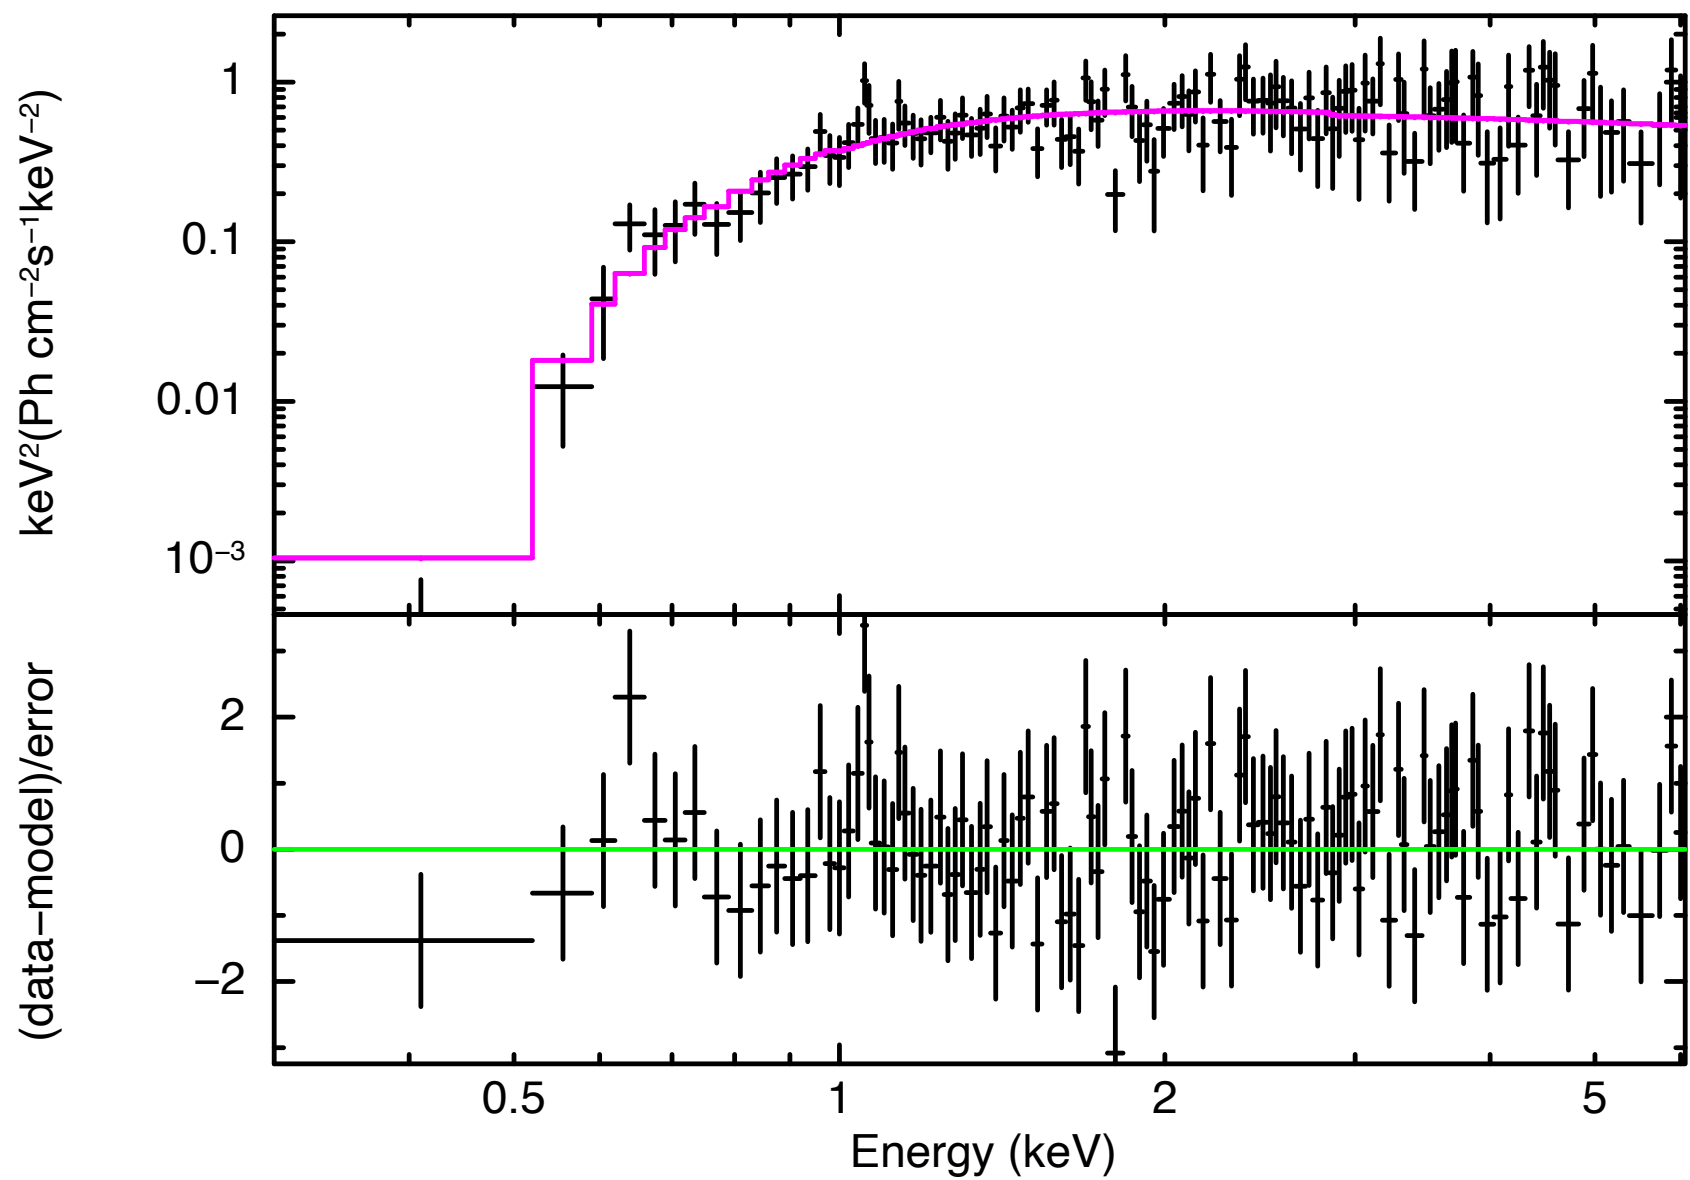

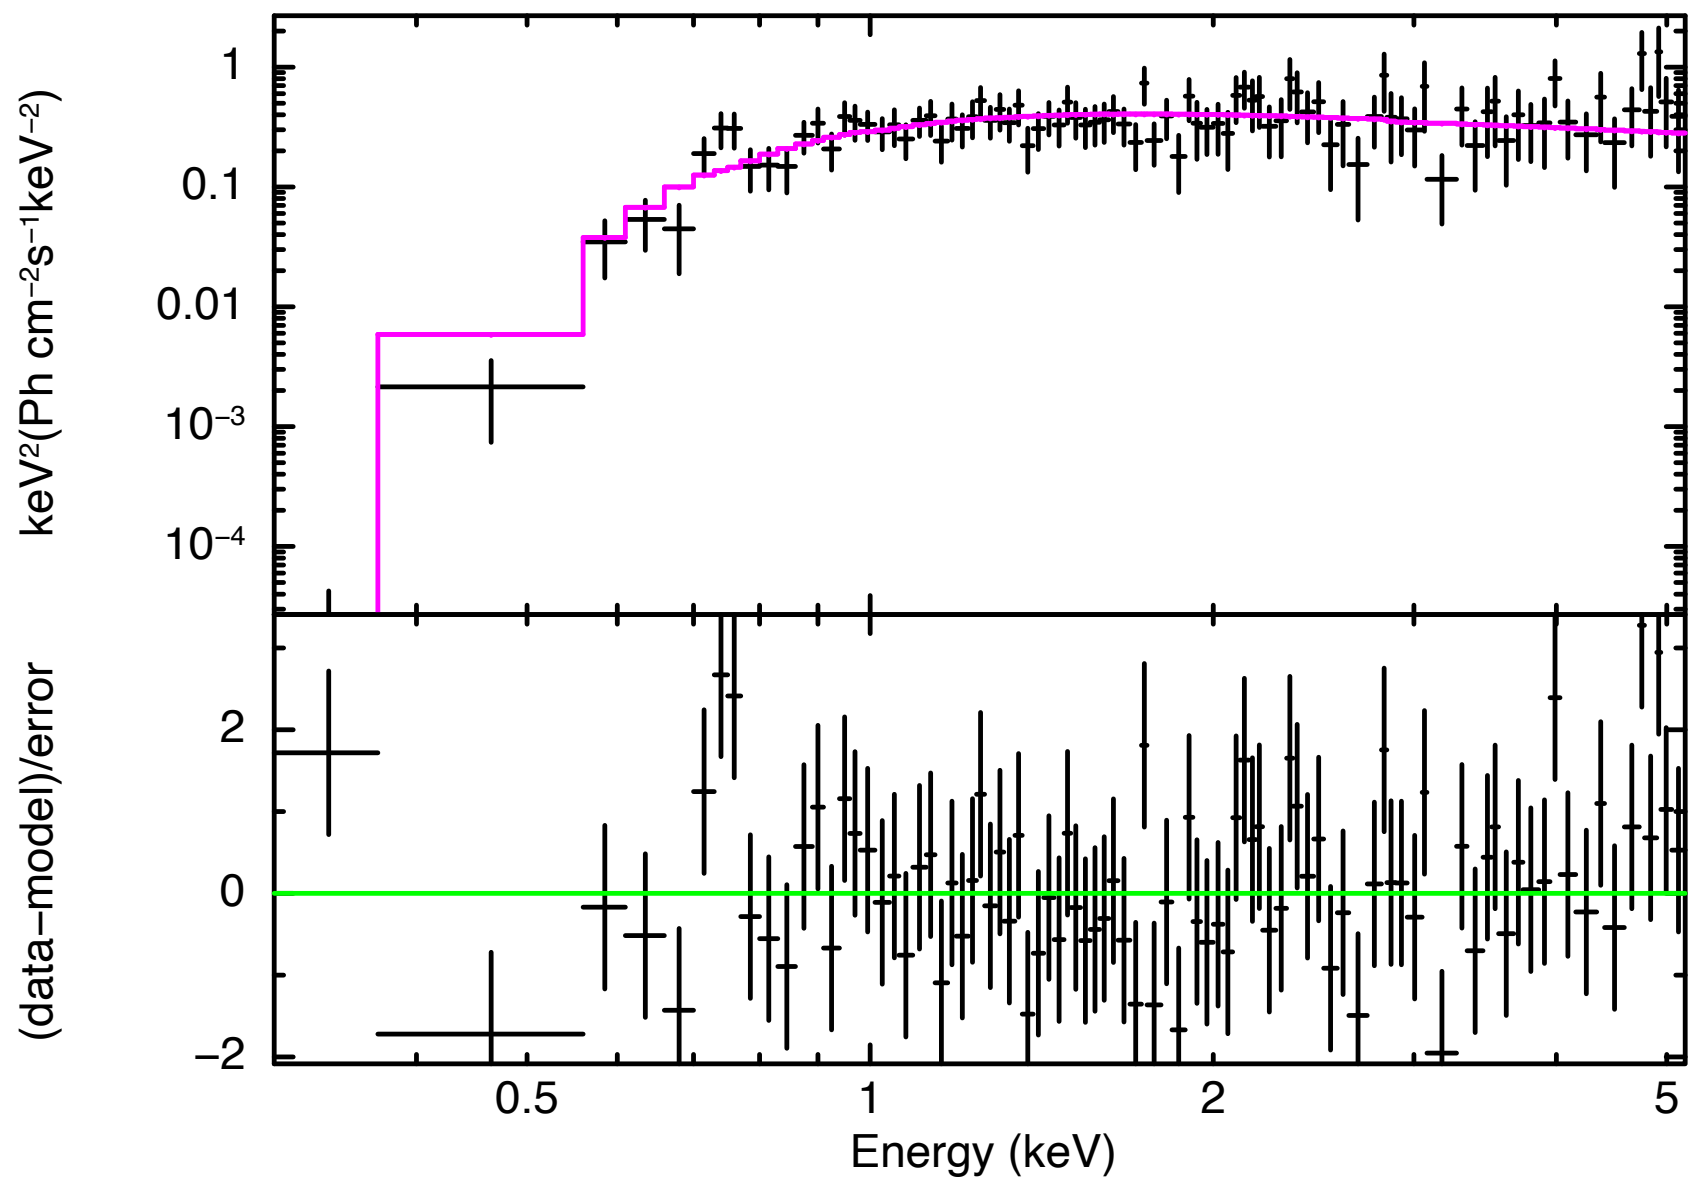

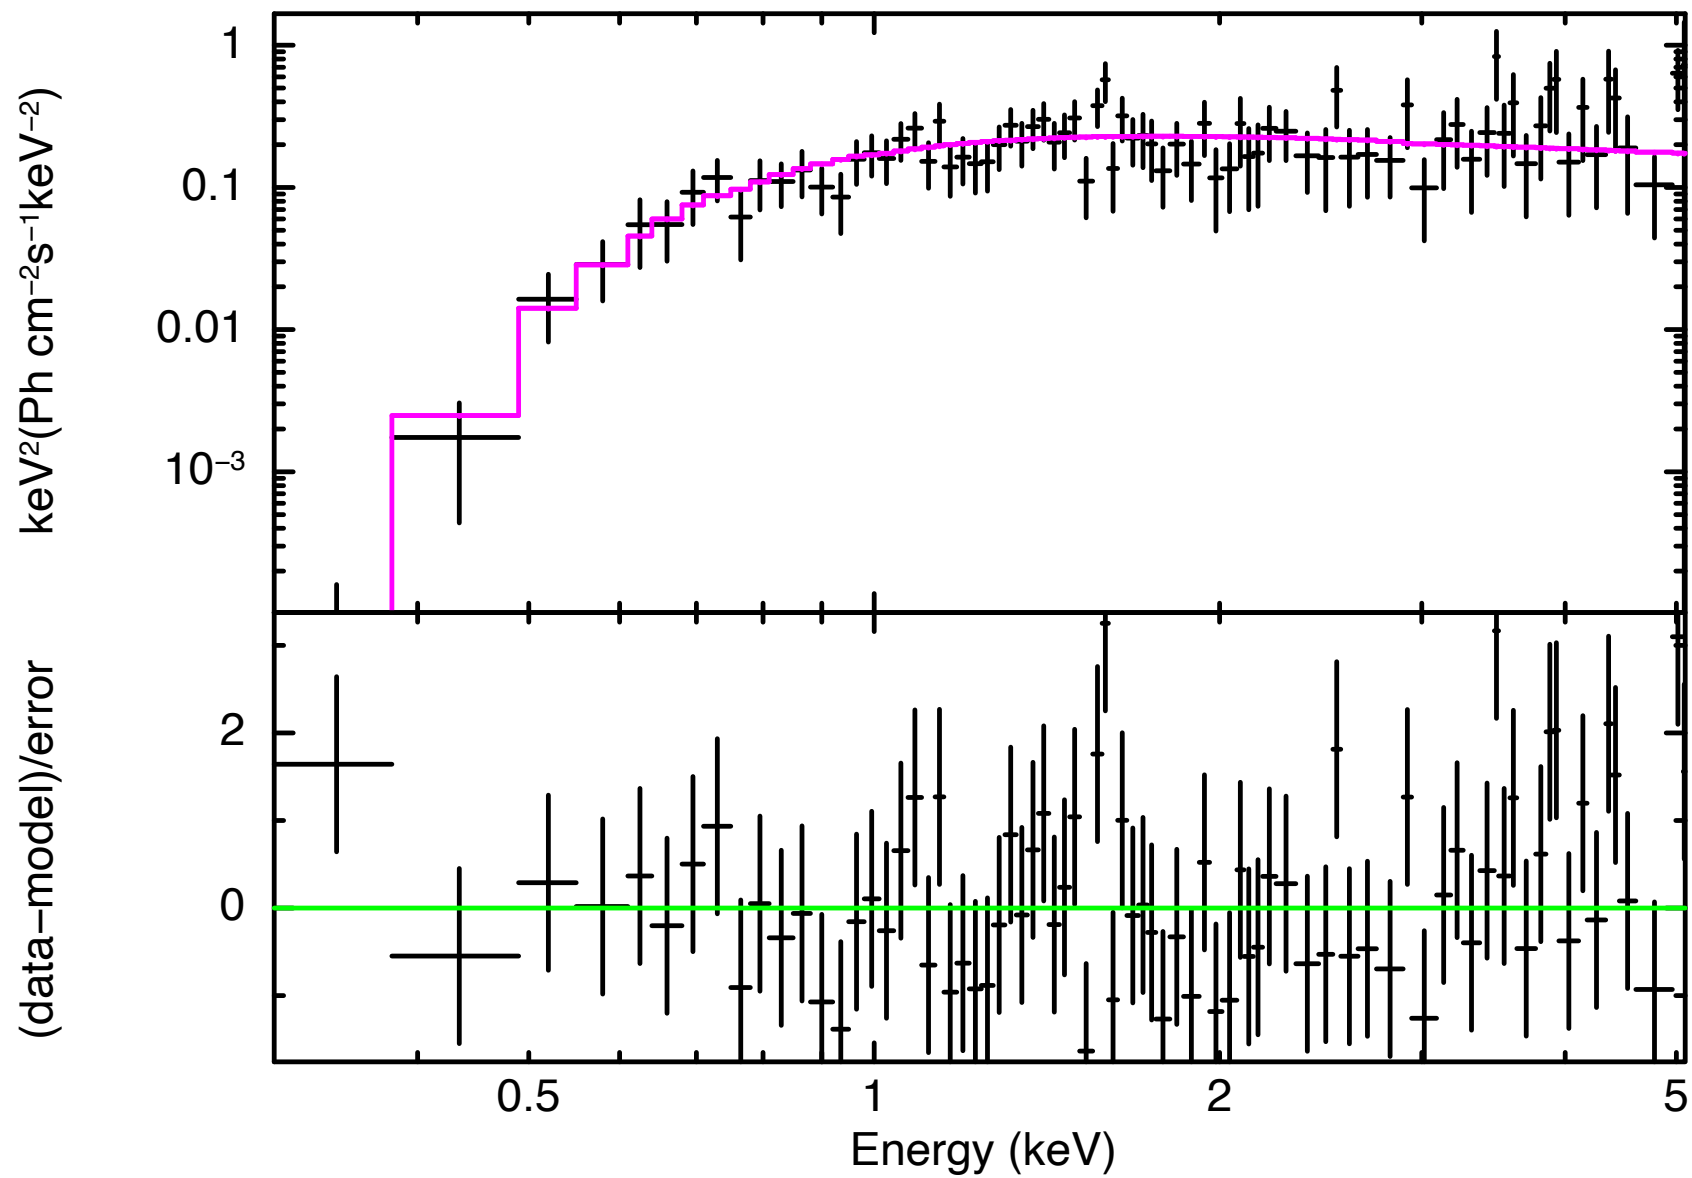

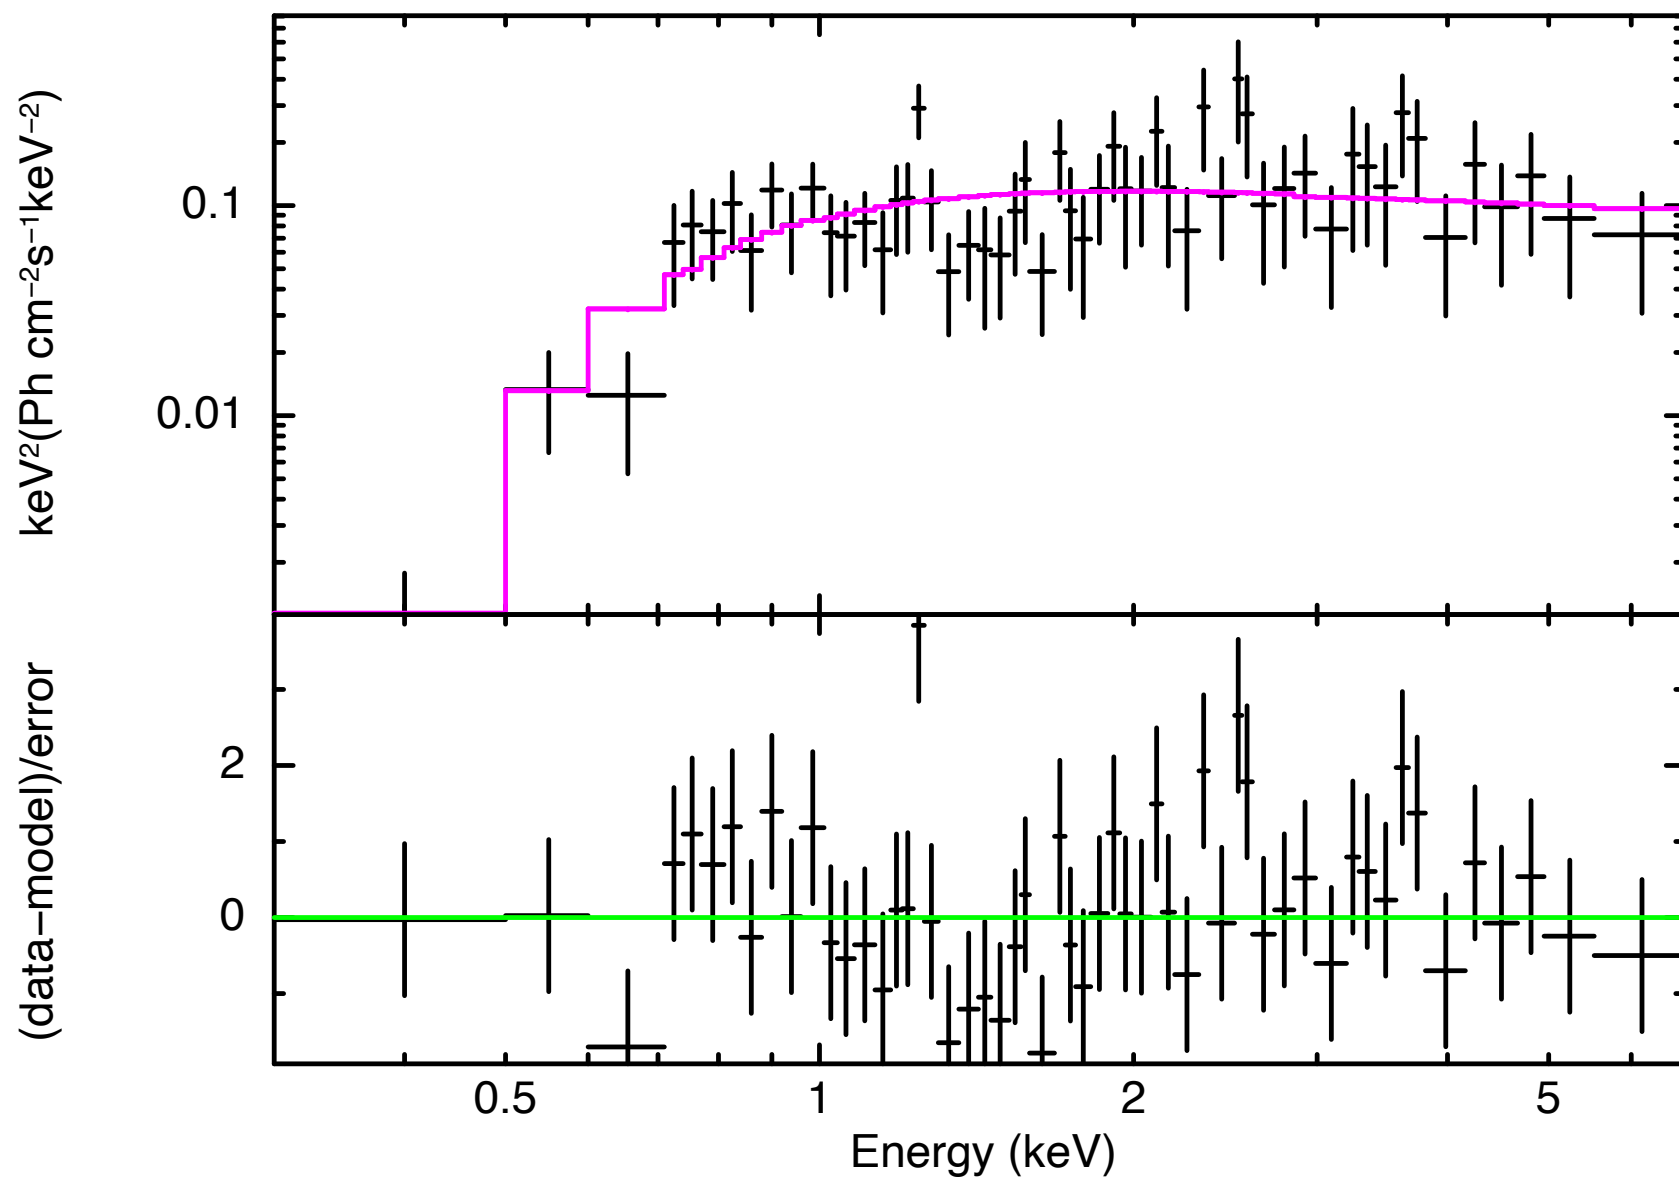

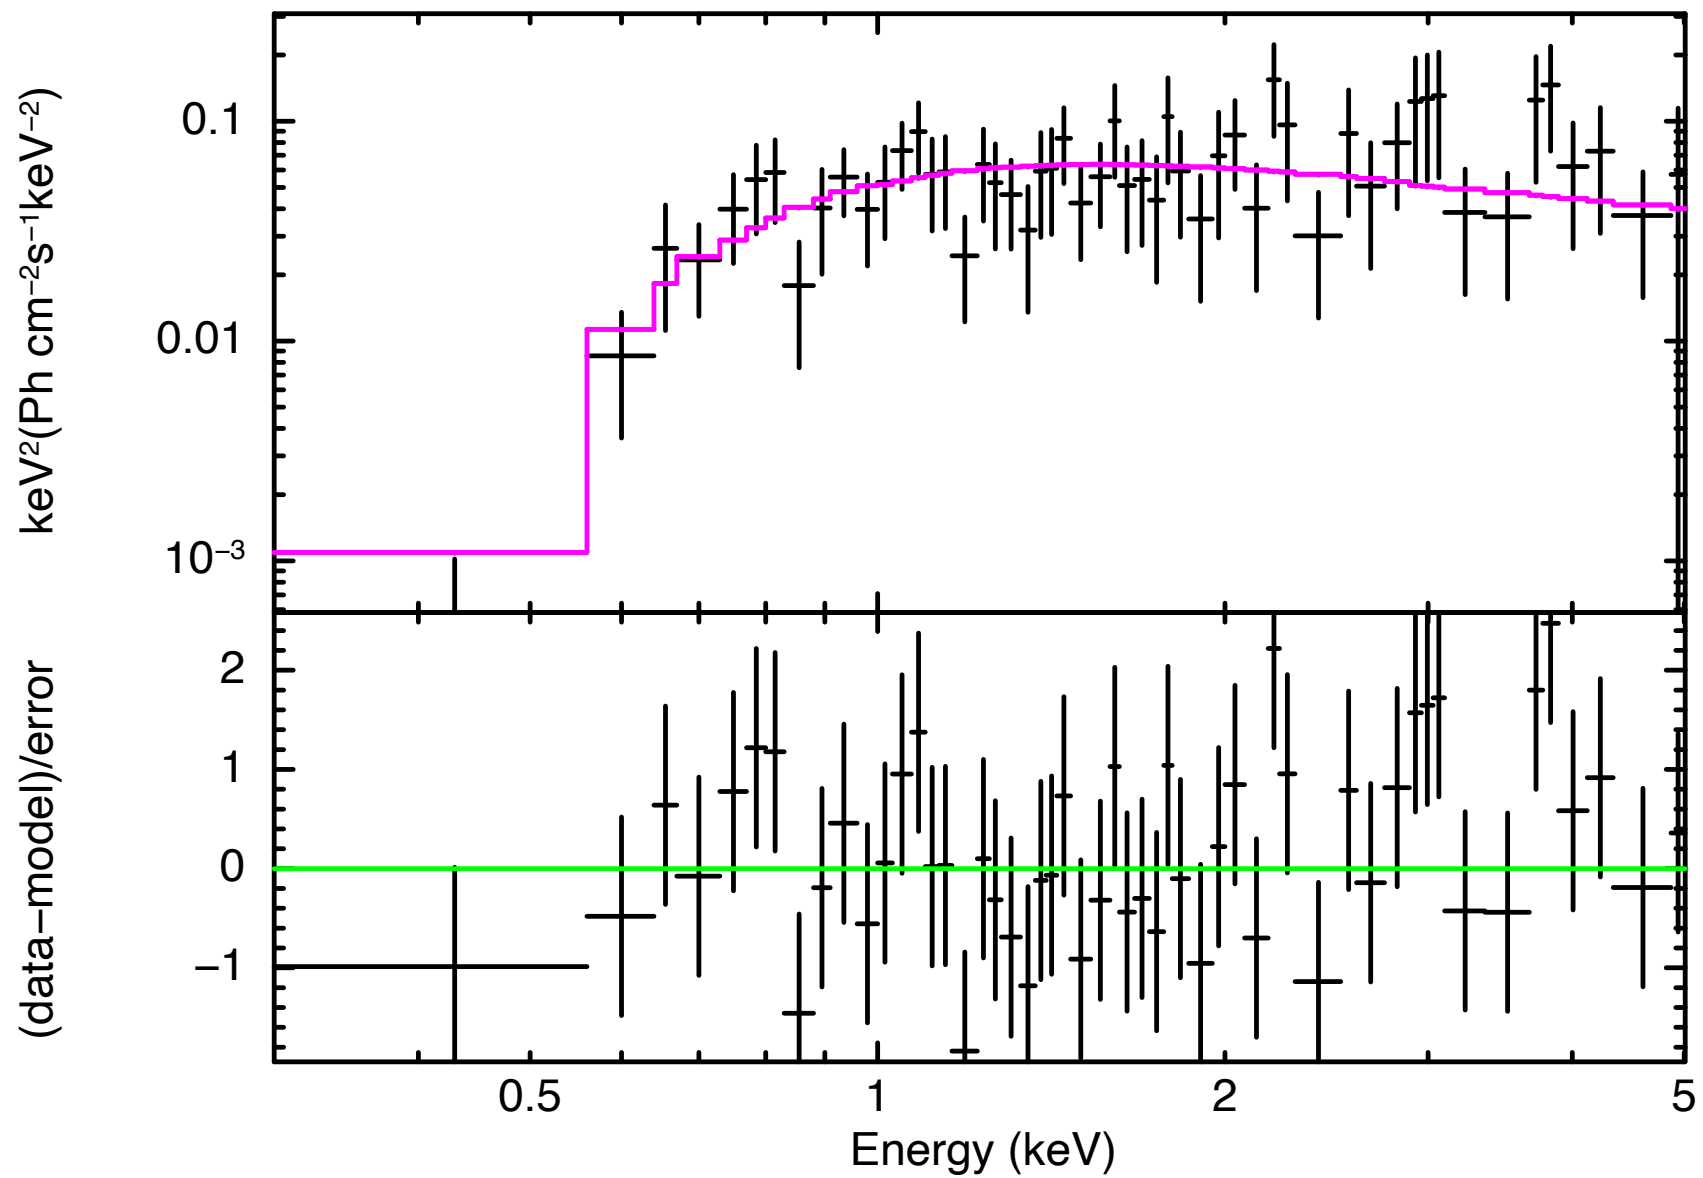

Supplement: Supplementary file 2 [file GRB070306_fits.pdf]
