# Supplementary material for: Investigating time variability of X-ray absorption in Swift GRBs
Source: arXiv:2301.09292 source file (2023-01-23)

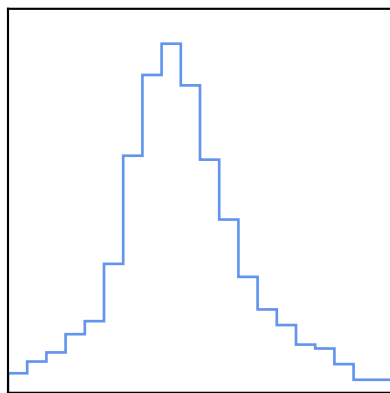

GRB071112C

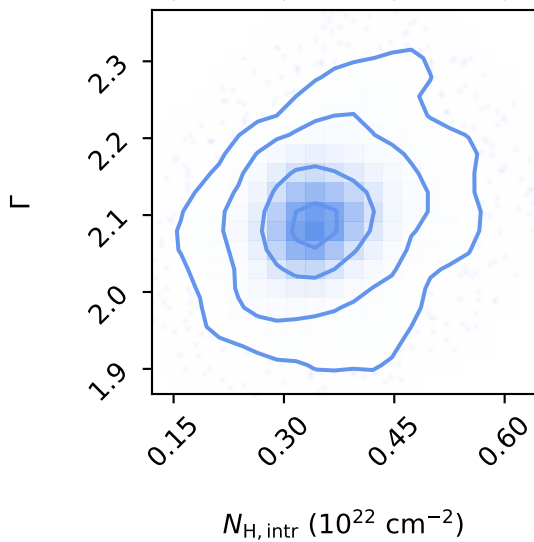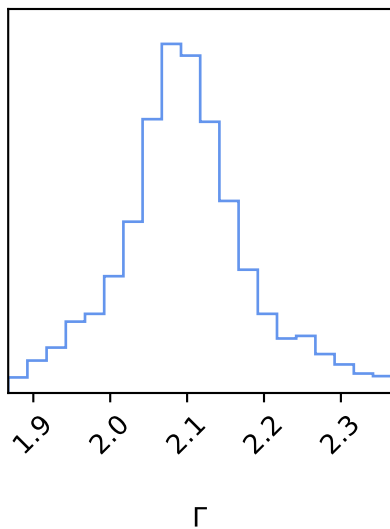

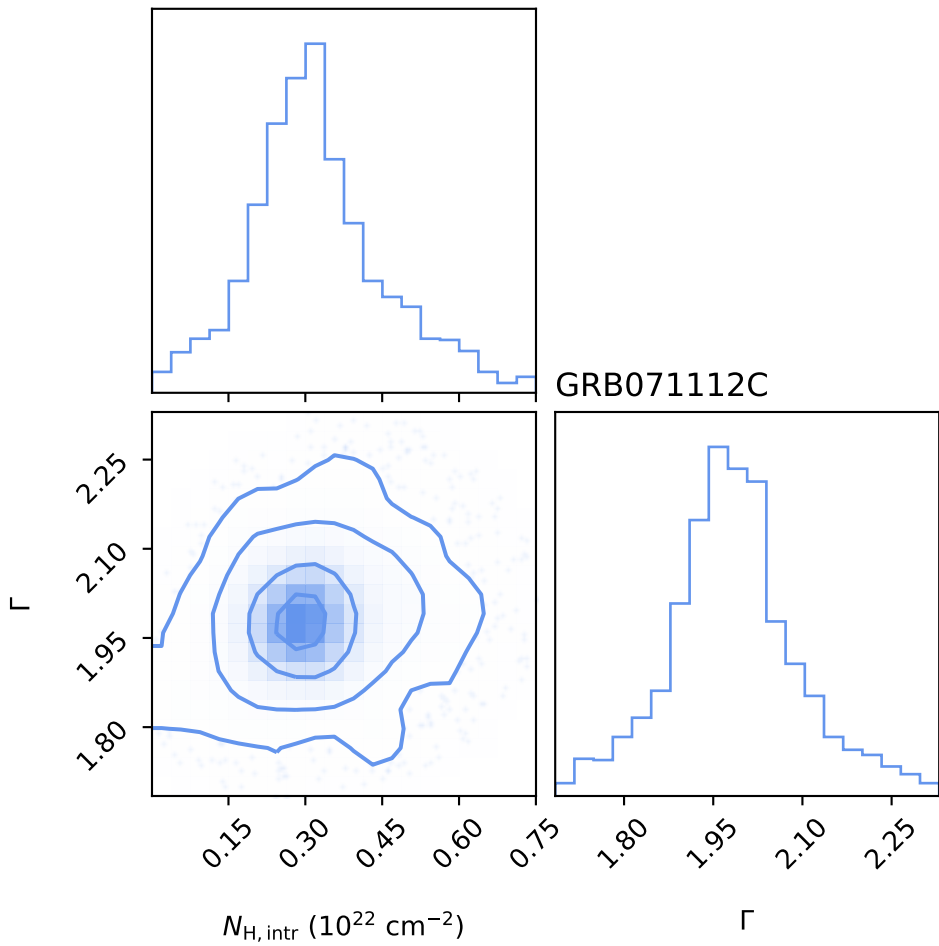

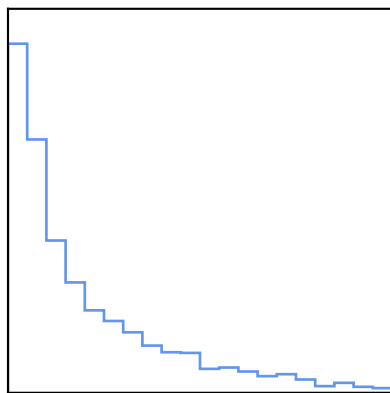

GRB071112C

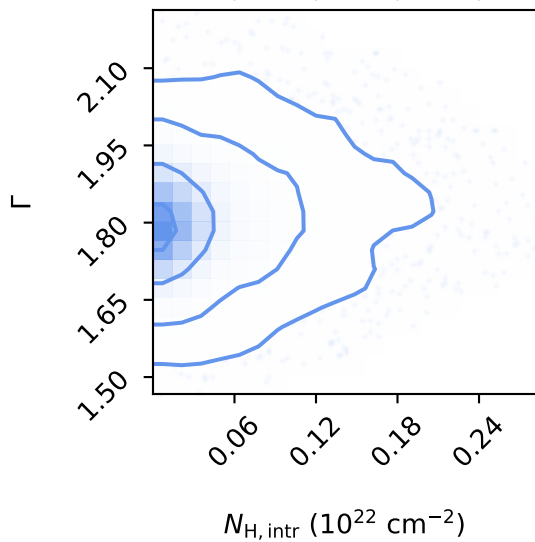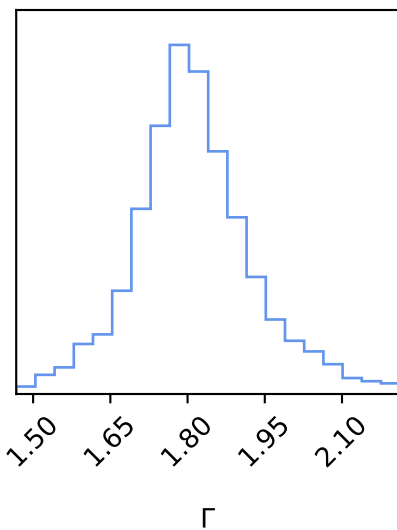

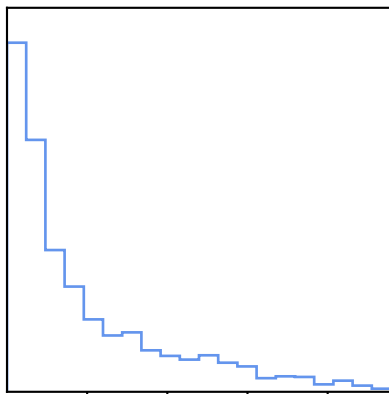

GRB071112C

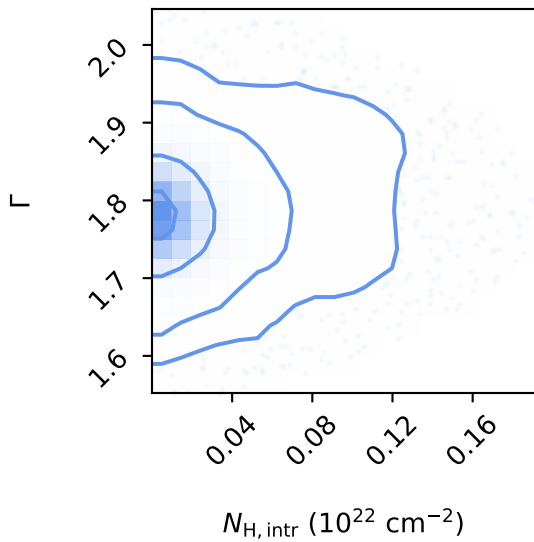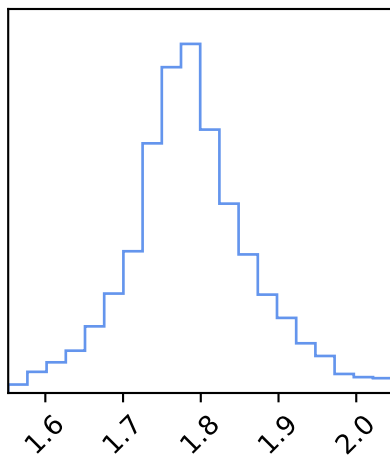

Supplement: Supplementary file 3 [file GRB071112C_cornerplot.pdf]
