# Supplementary material for: Investigating time variability of X-ray absorption in Swift GRBs
Source: arXiv:2301.09292 source file (2023-01-23)

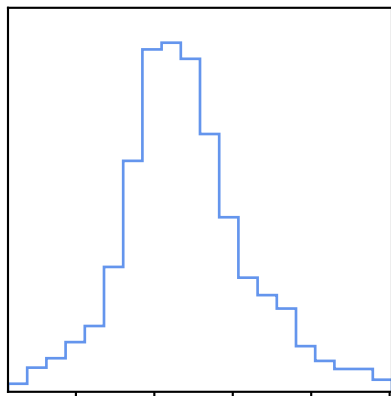

GRB081007

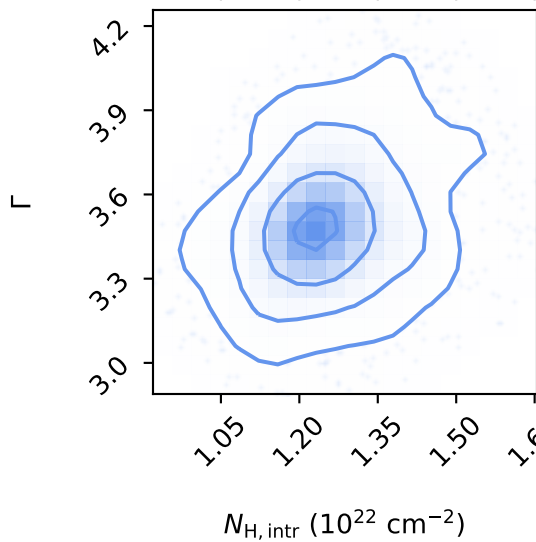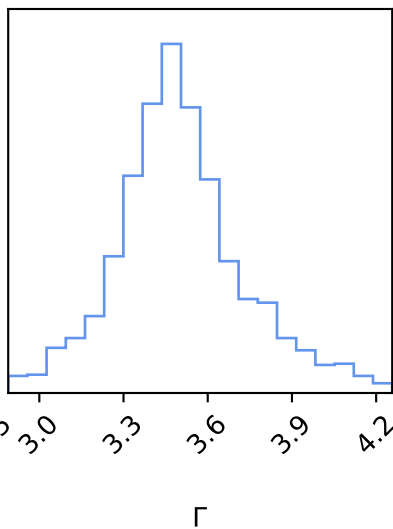

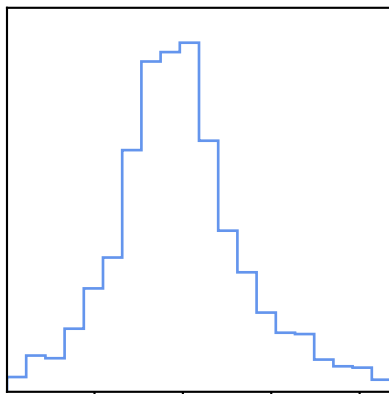

GRB081007

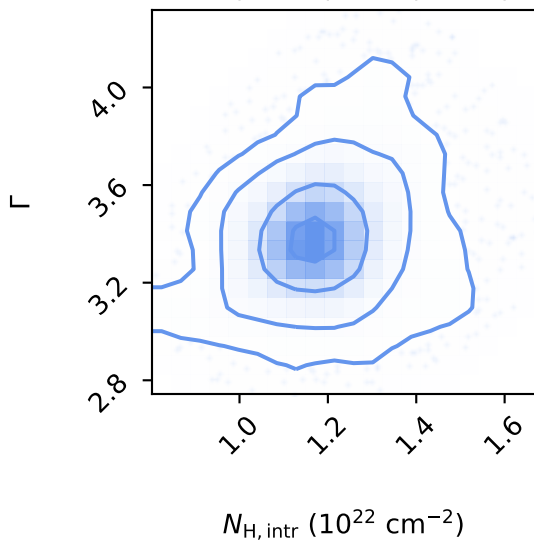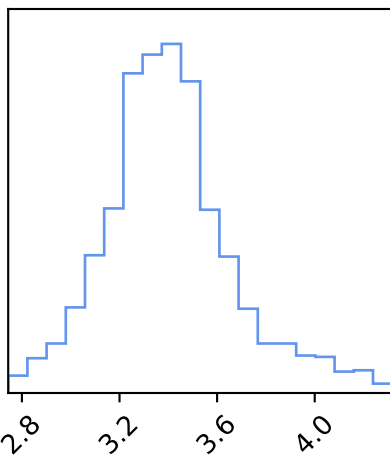

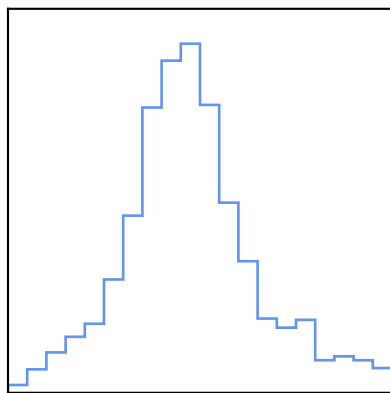

GRB081007

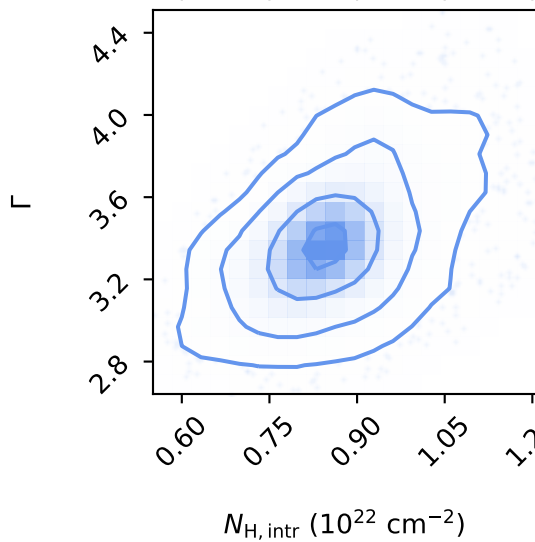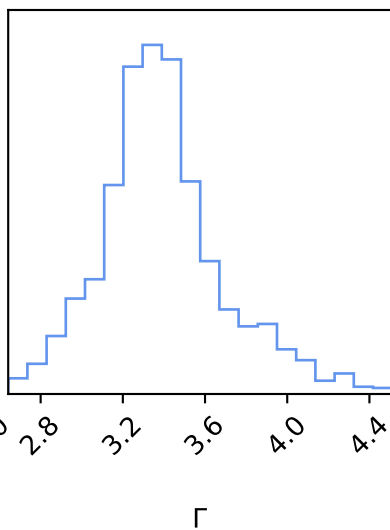

Supplement: Supplementary file 5 [file GRB081007_cornerplot.pdf]
