# Supplementary material for: Investigating time variability of X-ray absorption in Swift GRBs
Source: arXiv:2301.09292 source file (2023-01-23)

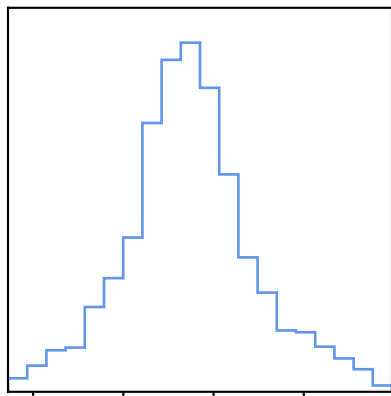

GRB090926B

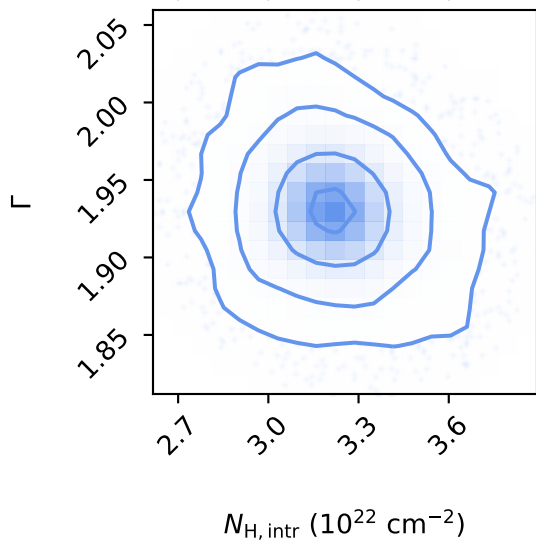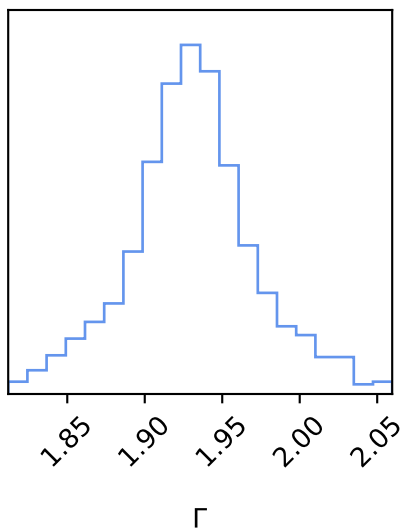

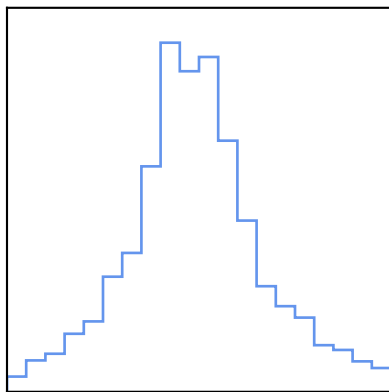

GRB090926B

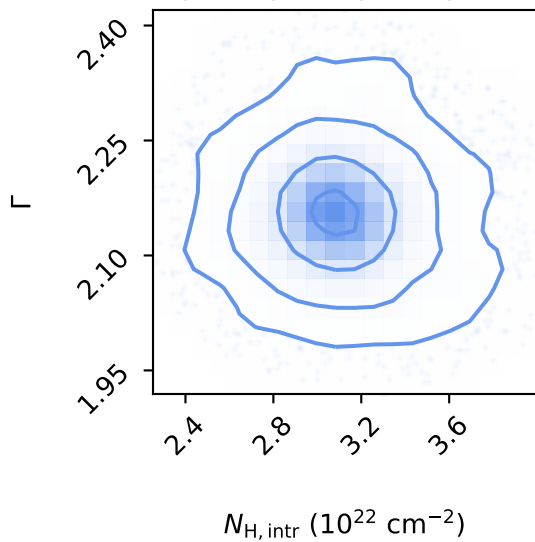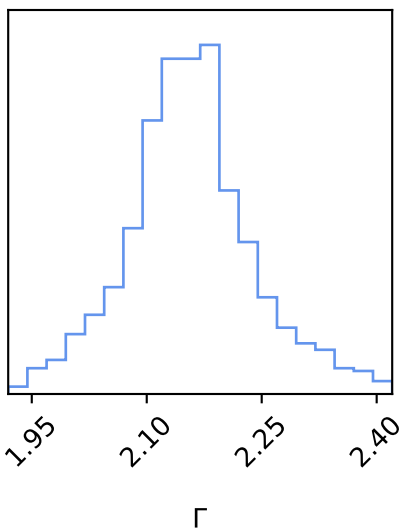

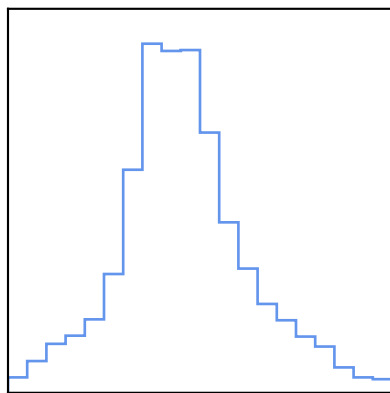

GRB090926B

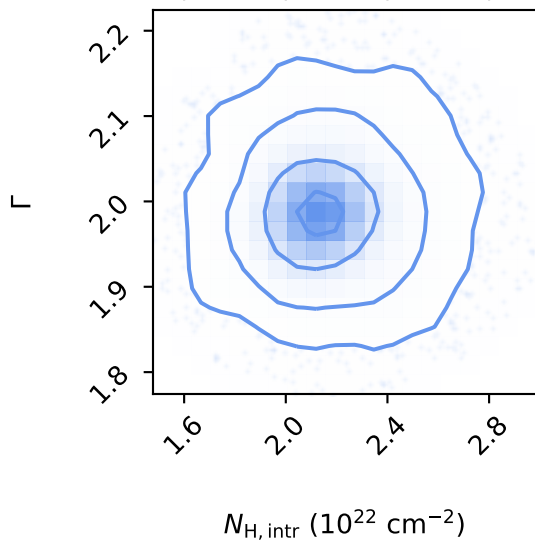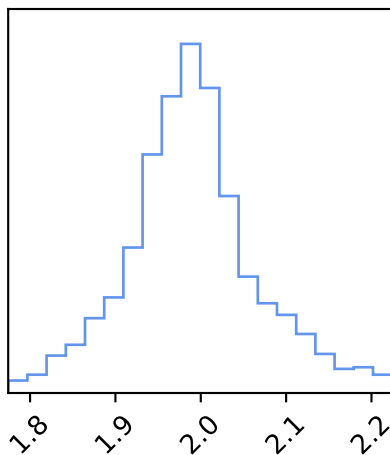

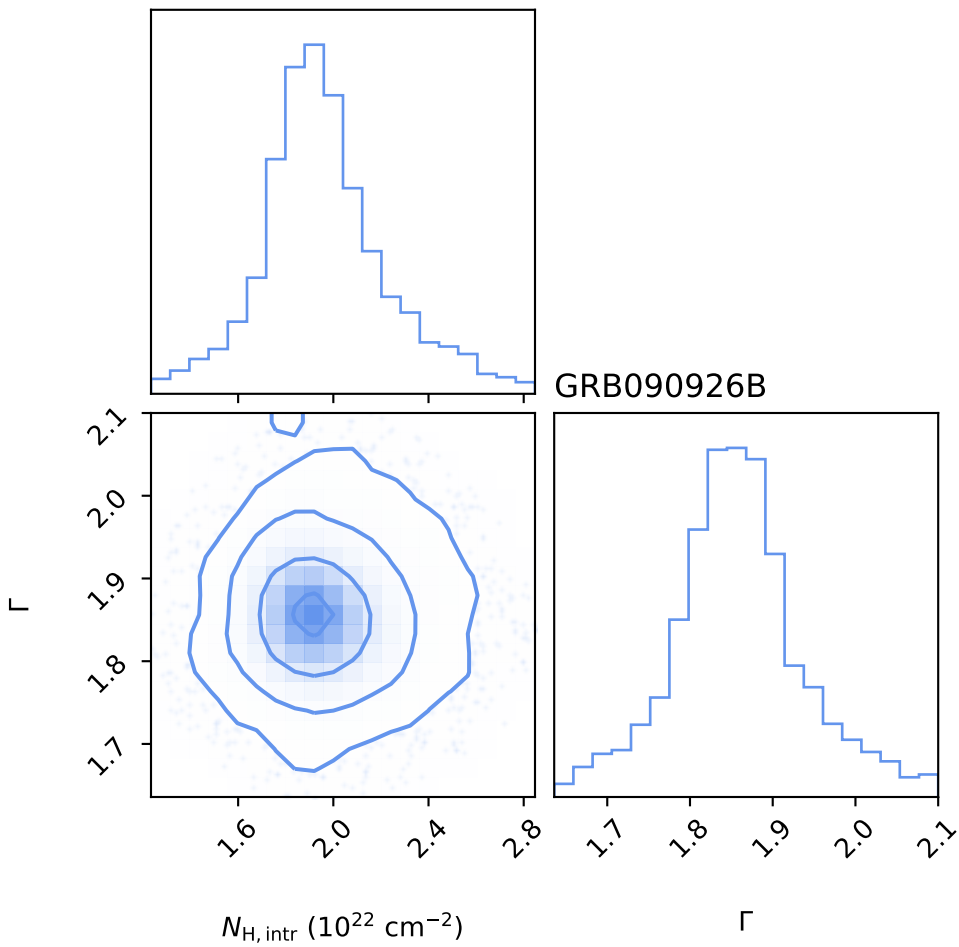

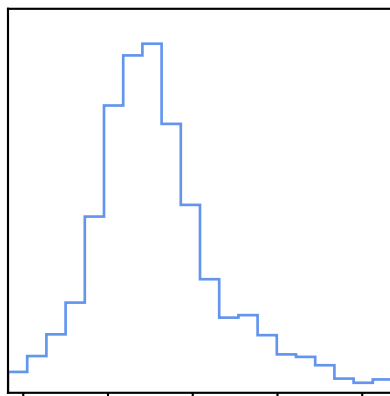

GRB090926B

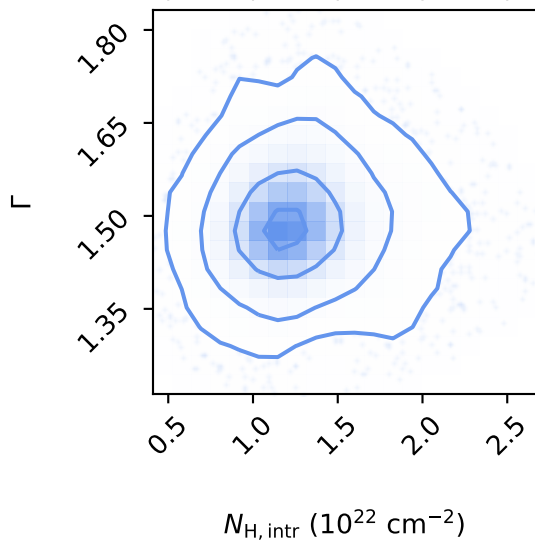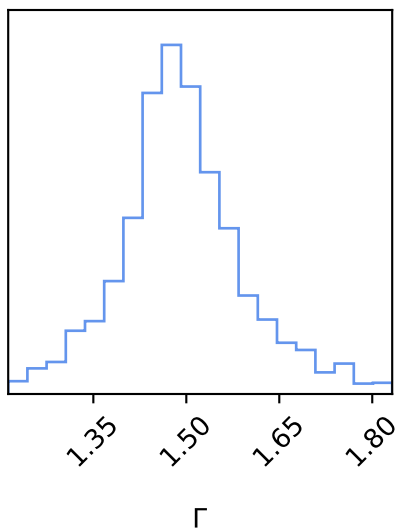

Supplement: Supplementary file 7 [file GRB090926B_cornerplot.pdf]
