# Supplementary material for: Investigating time variability of X-ray absorption in Swift GRBs
Source: arXiv:2301.09292 source file (2023-01-23)

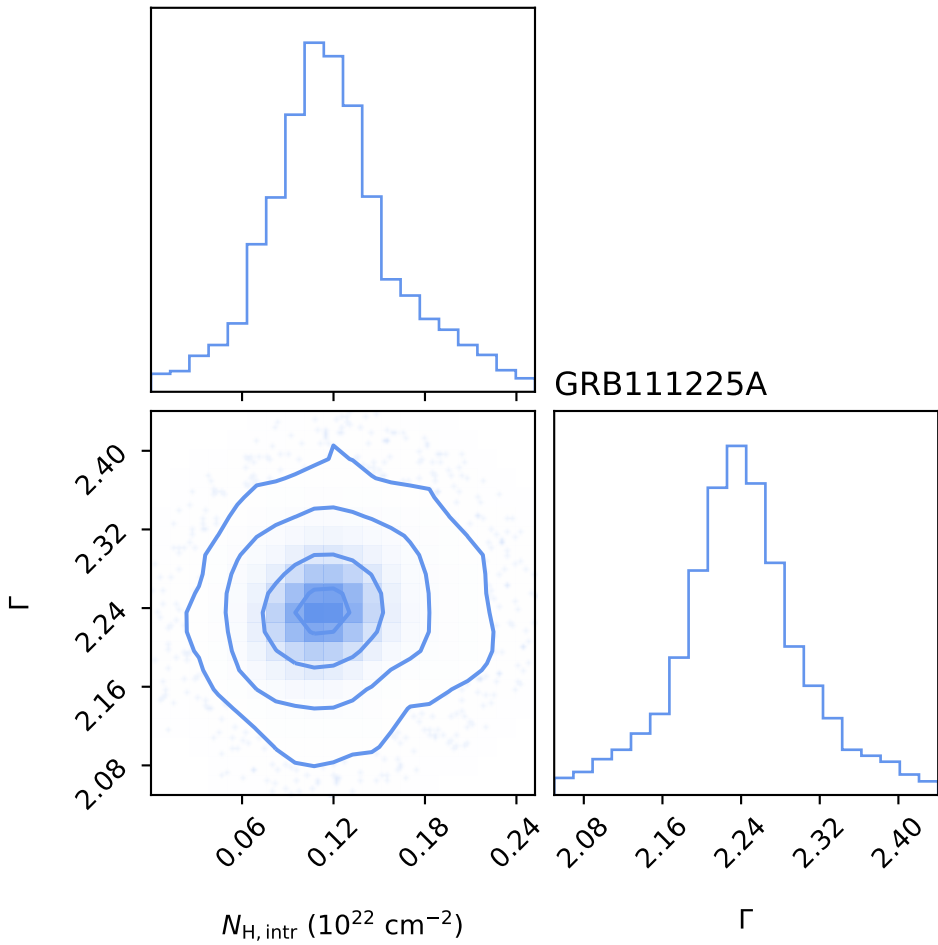

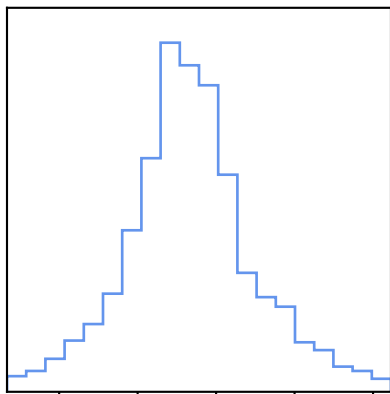

GRB111225A

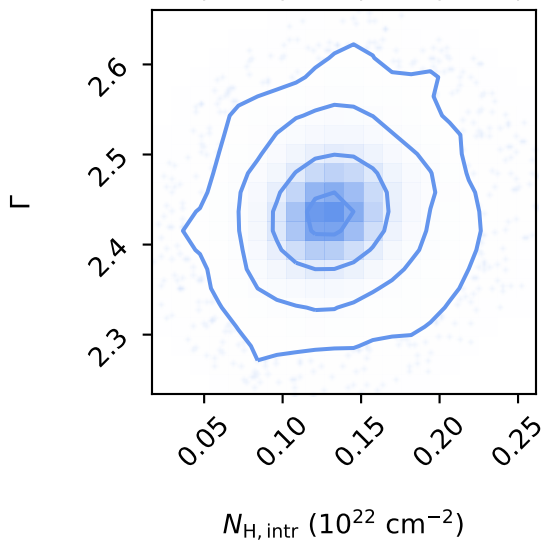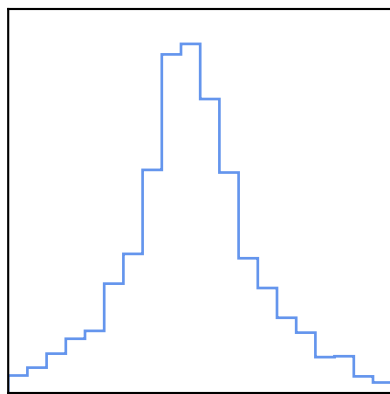

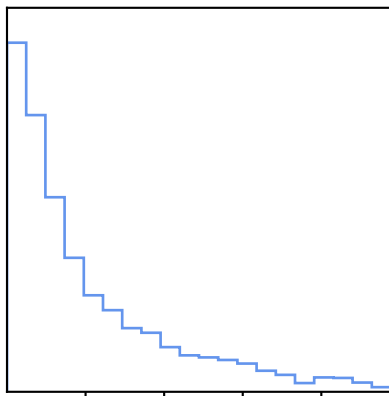

GRB111225A

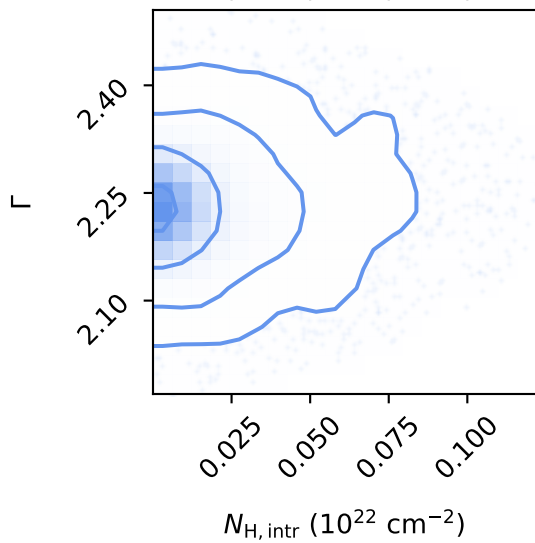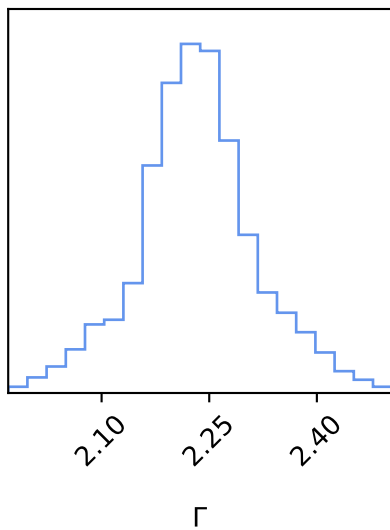

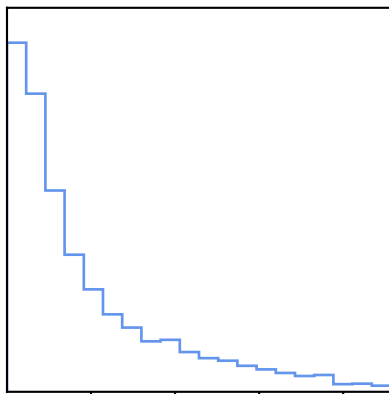

GRB111225A

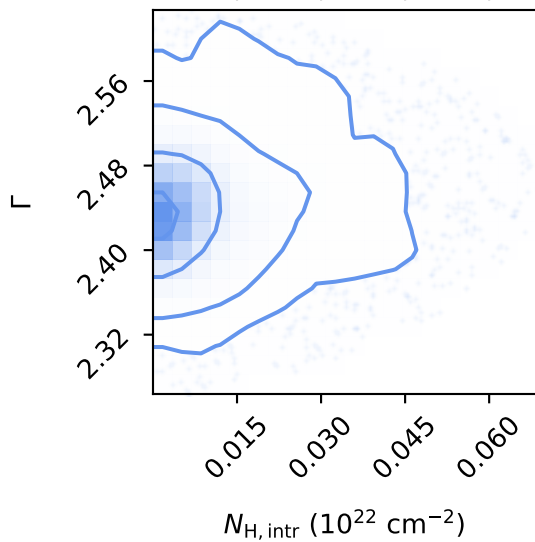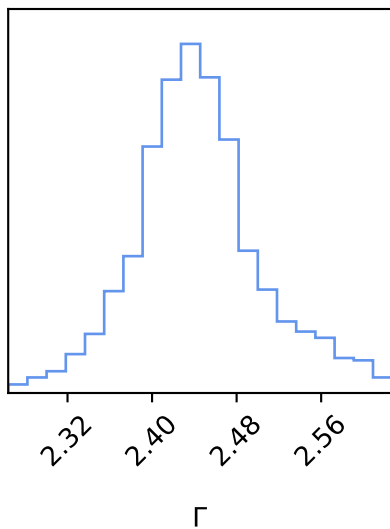

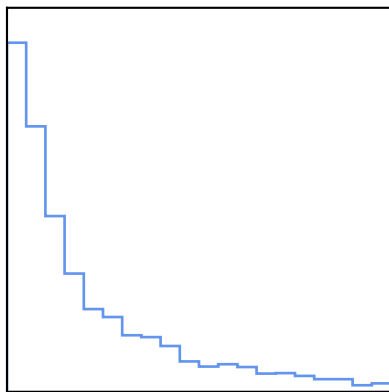

GRB111225A

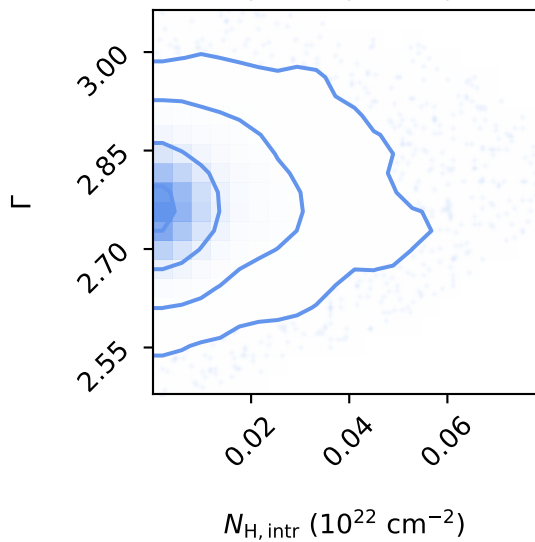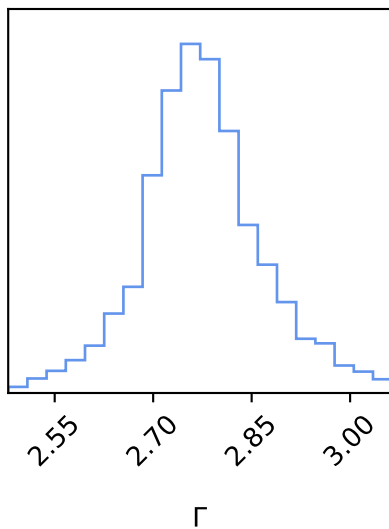

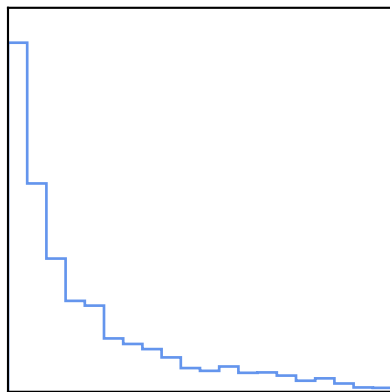

GRB111225A

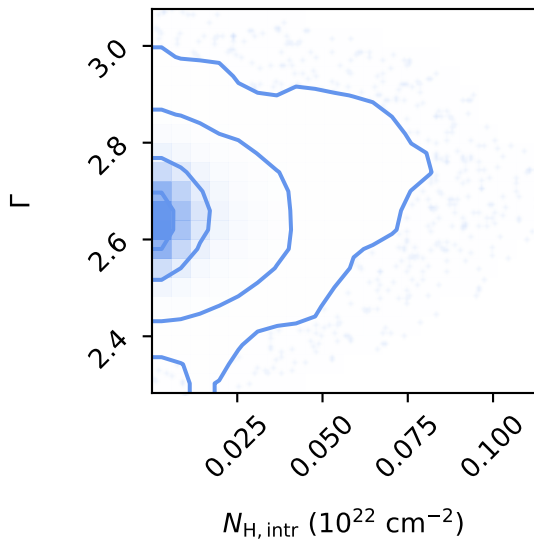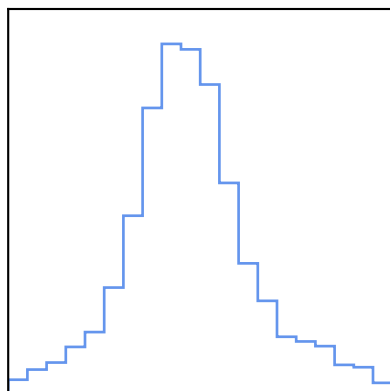

Supplement: Supplementary file 9 [file GRB111225A_cornerplot.pdf]
