# Supplementary material for: Investigating time variability of X-ray absorption in Swift GRBs
Source: arXiv:2301.09292 source file (2023-01-23)

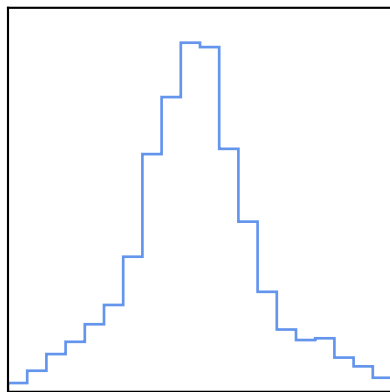

GRB170607A

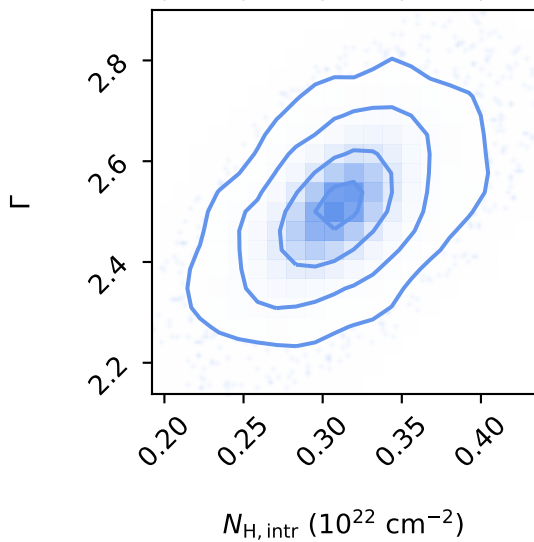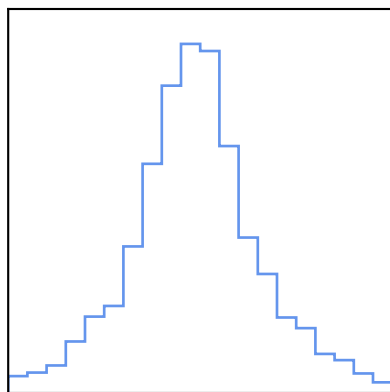

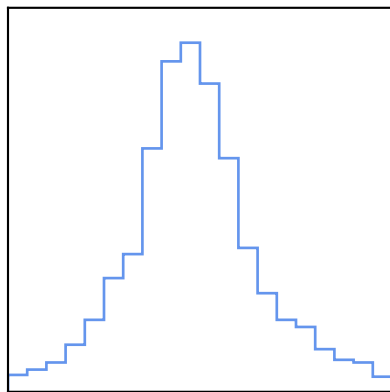

GRB170607A

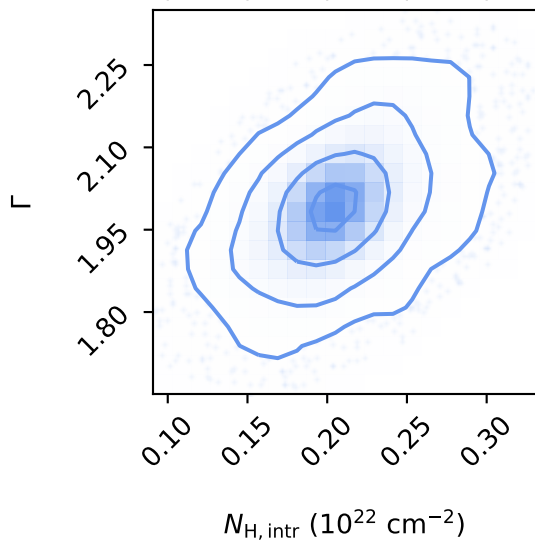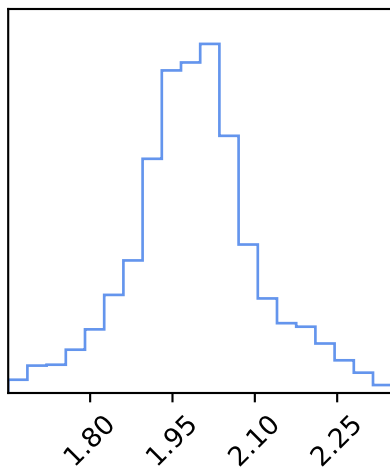

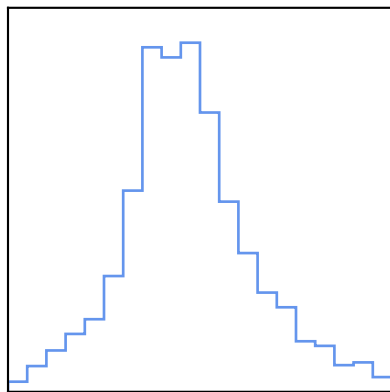

GRB170607A

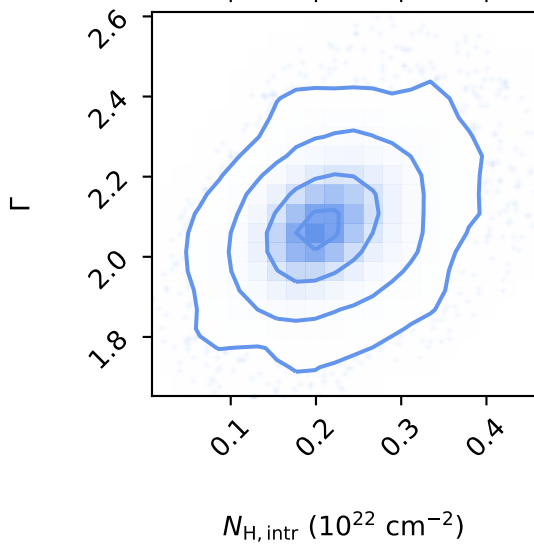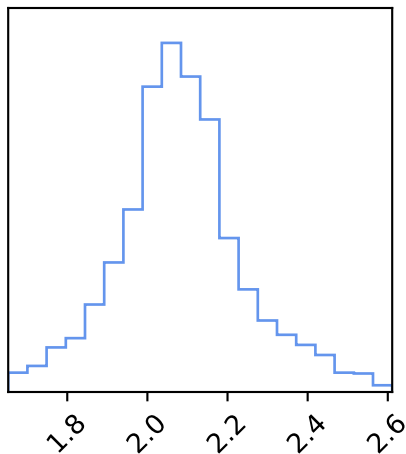

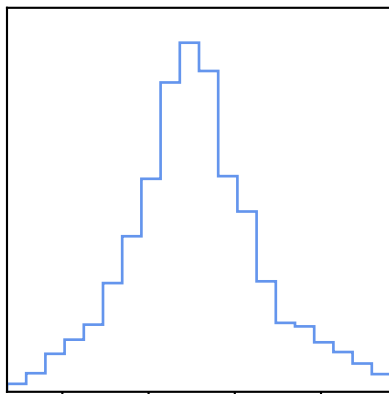

GRB170607A

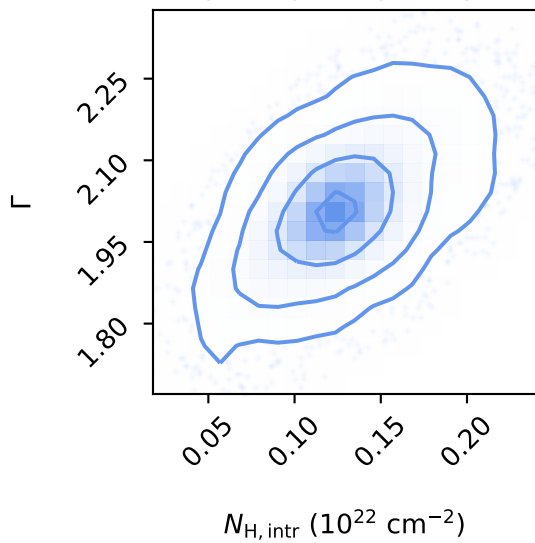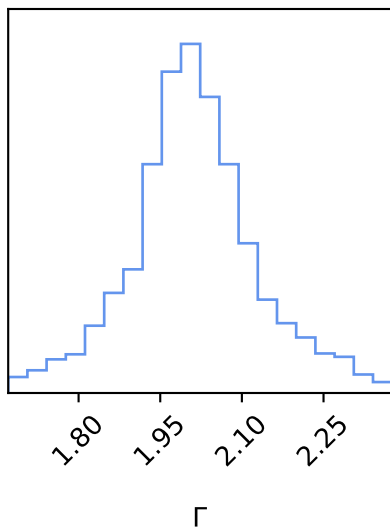

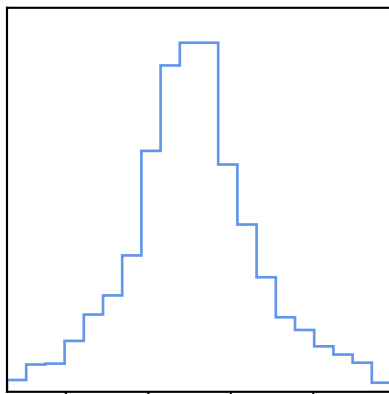

GRB170607A

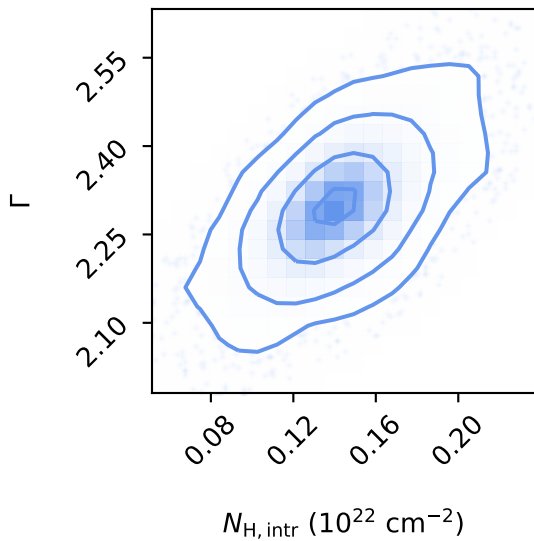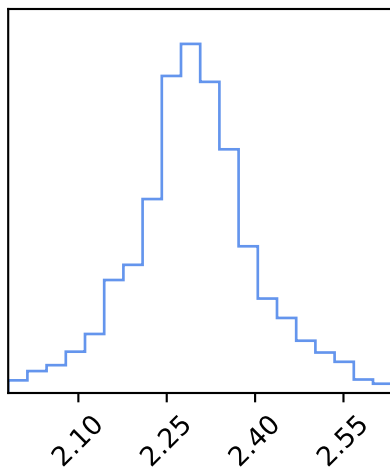

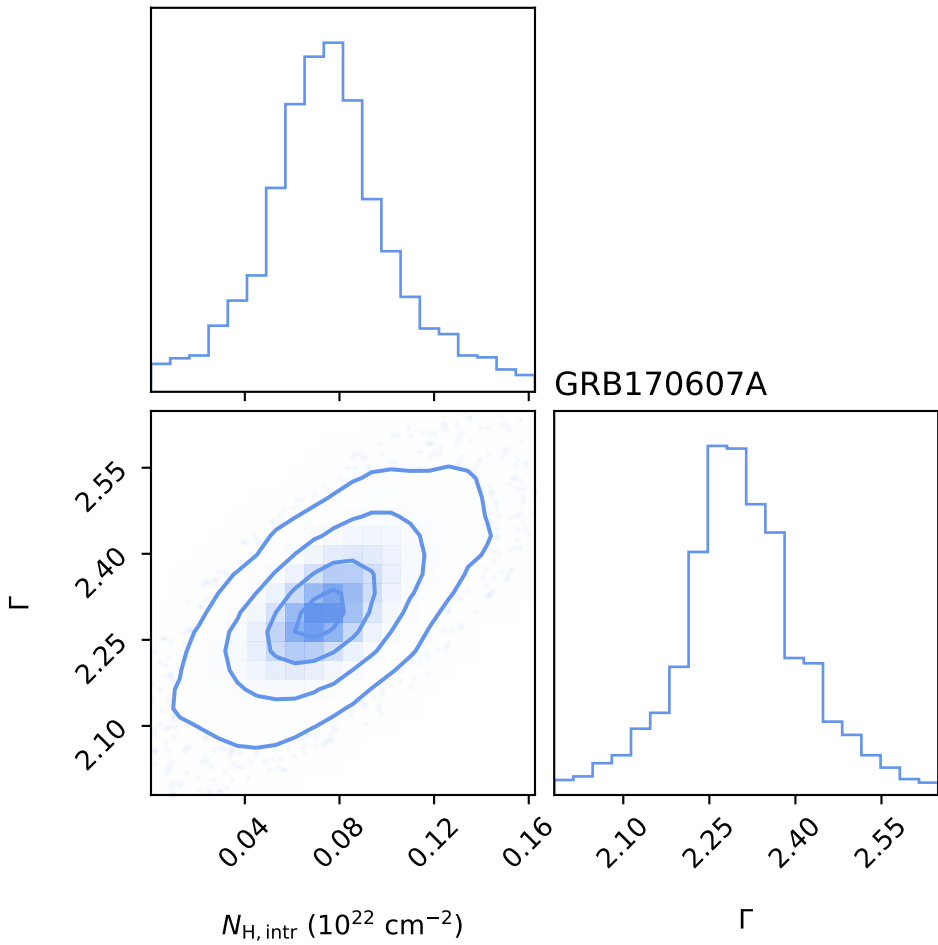

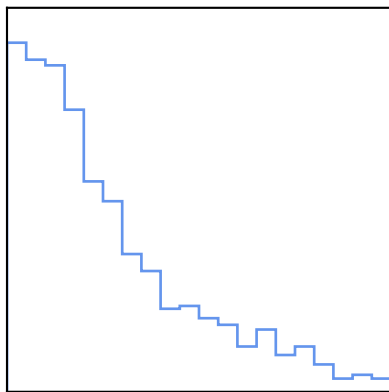

GRB170607A

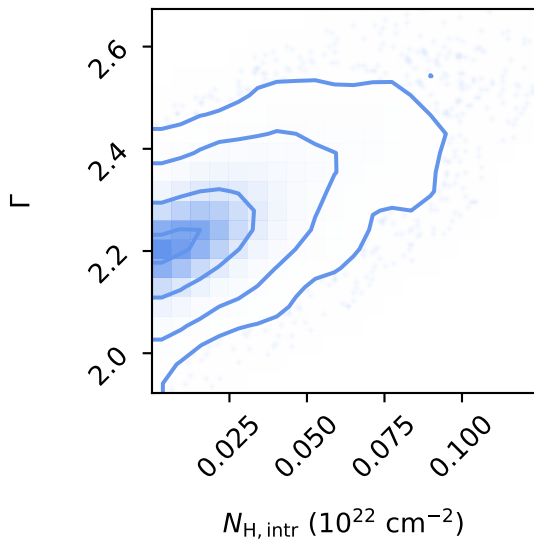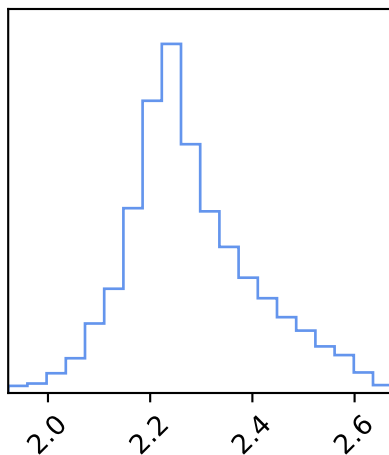

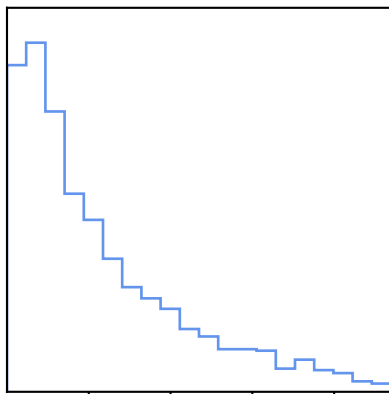

GRB170607A

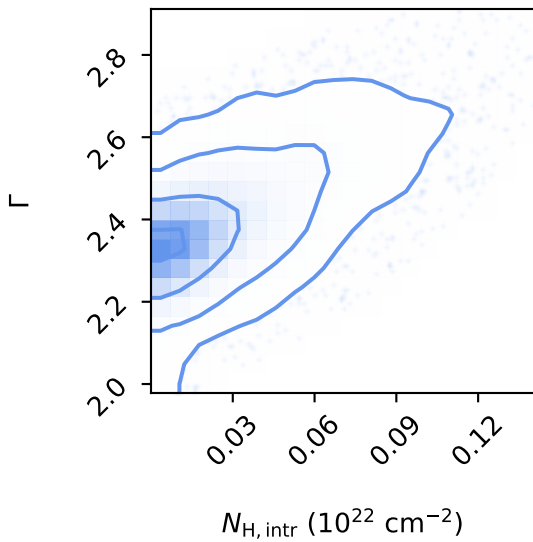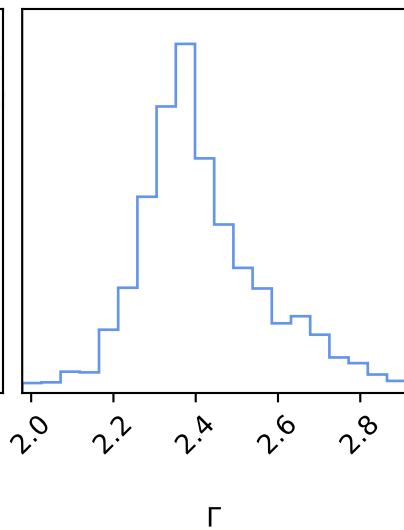



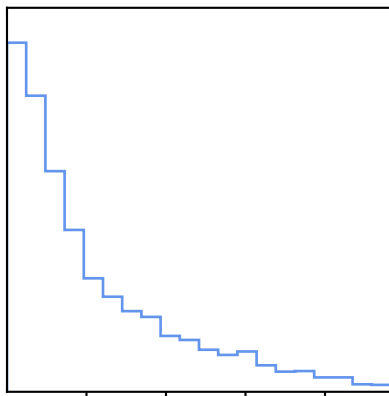

GRB170607A

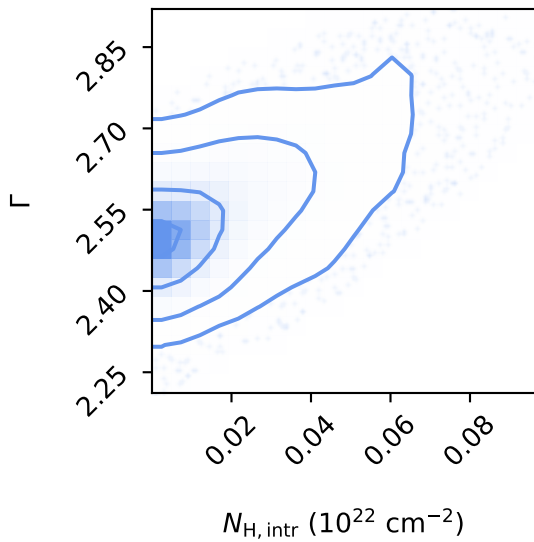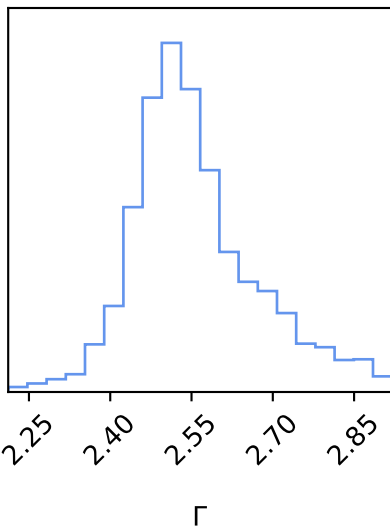

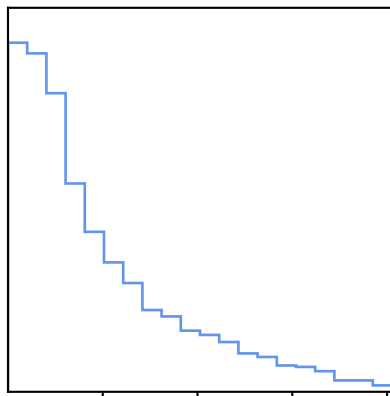

GRB170607A

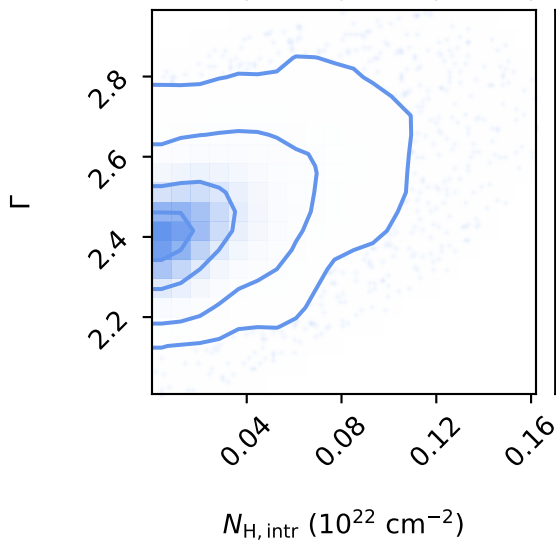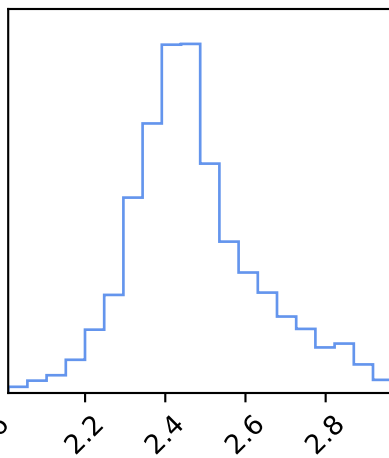

Supplement: Supplementary file 11 [file GRB170607A_cornerplot.pdf]
