# Supplementary material for: Investigating time variability of X-ray absorption in Swift GRBs
Source: arXiv:2301.09292 source file (2023-01-23)

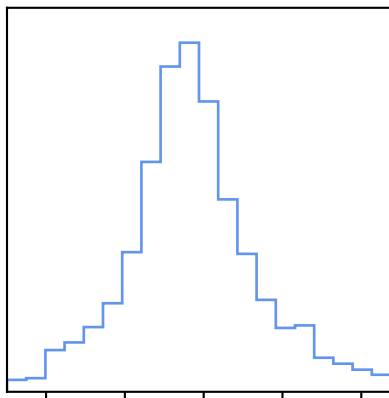

GRB171222A

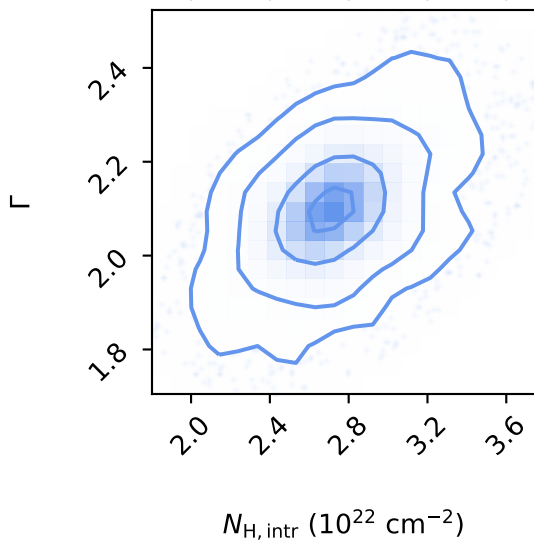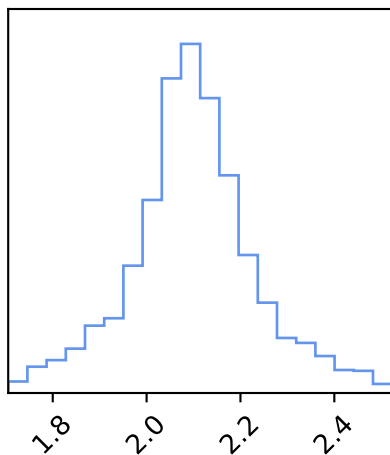

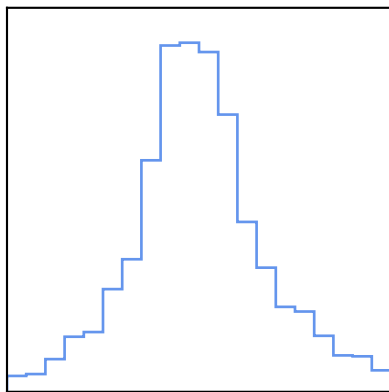

GRB171222A

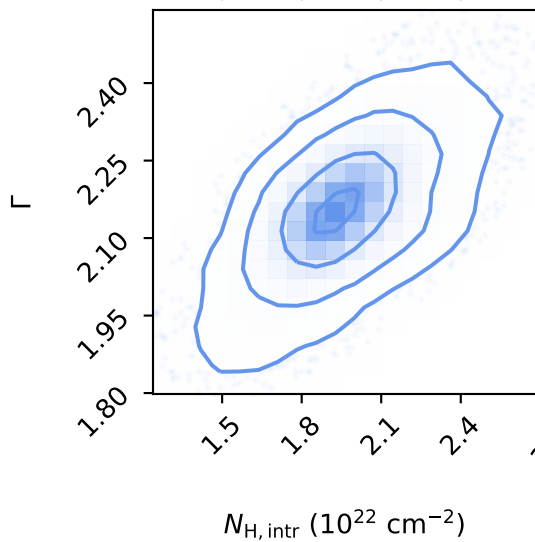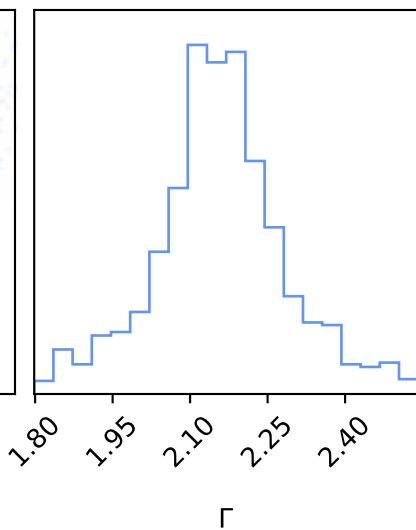

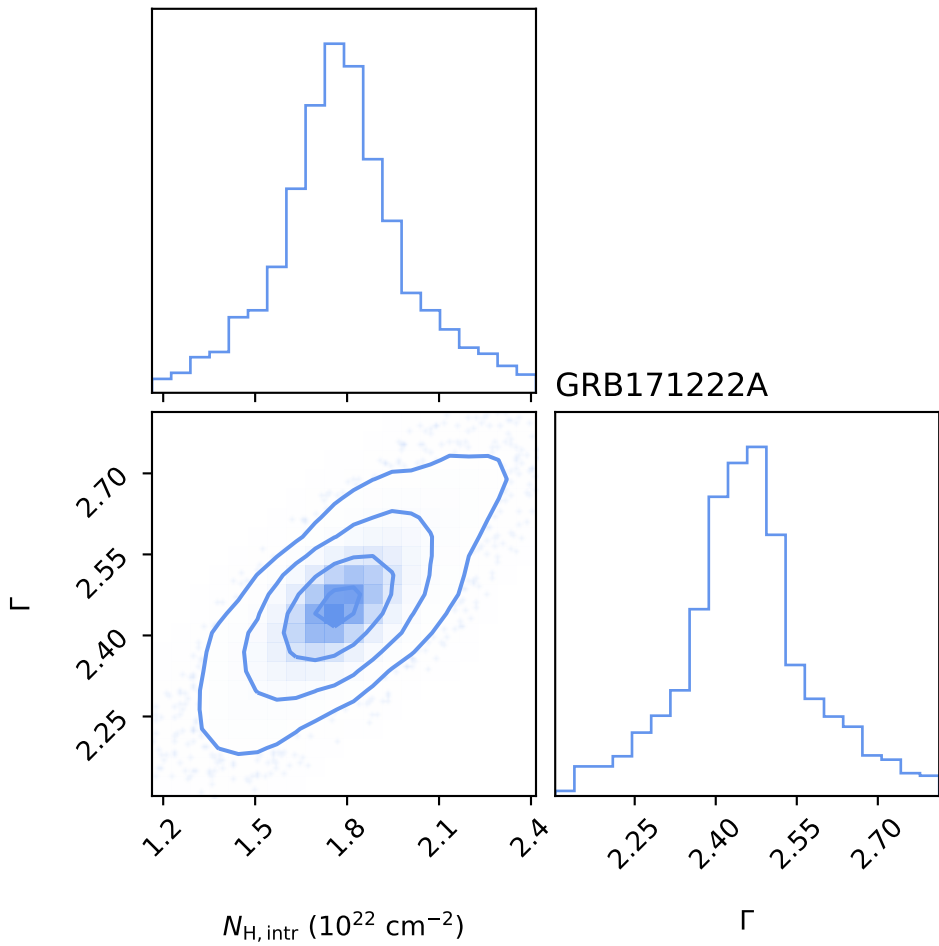

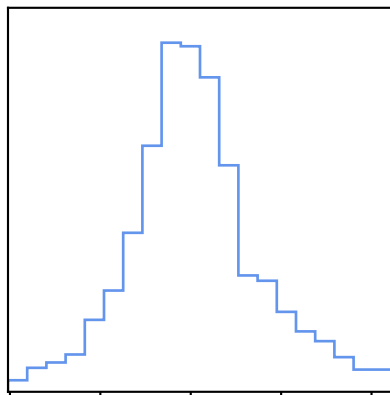

GRB171222A

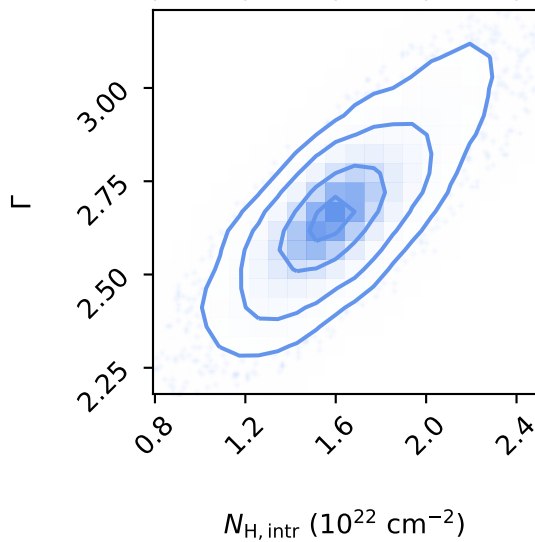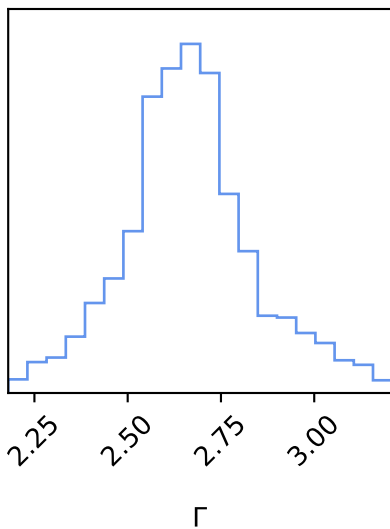

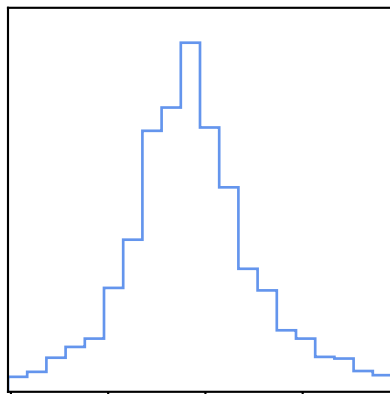

GRB171222A

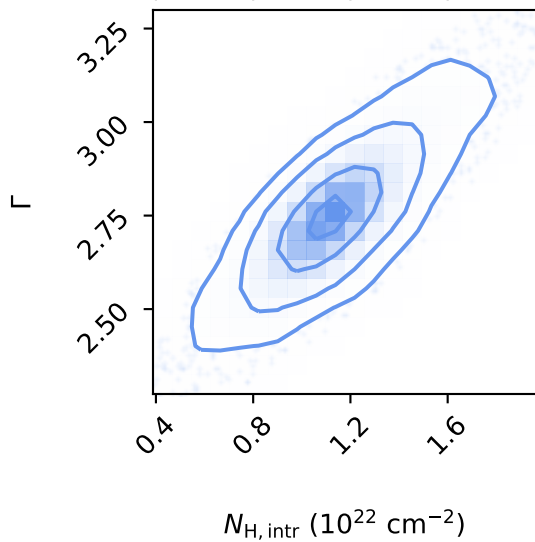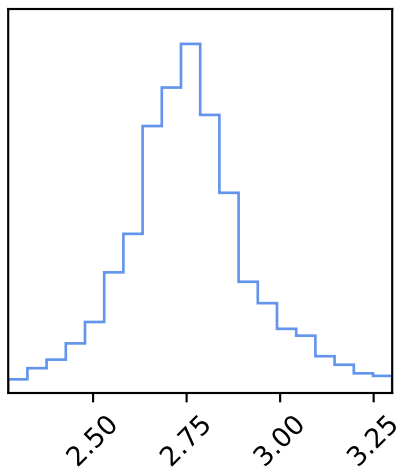

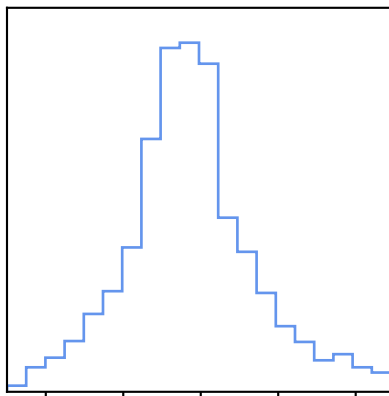

GRB171222A

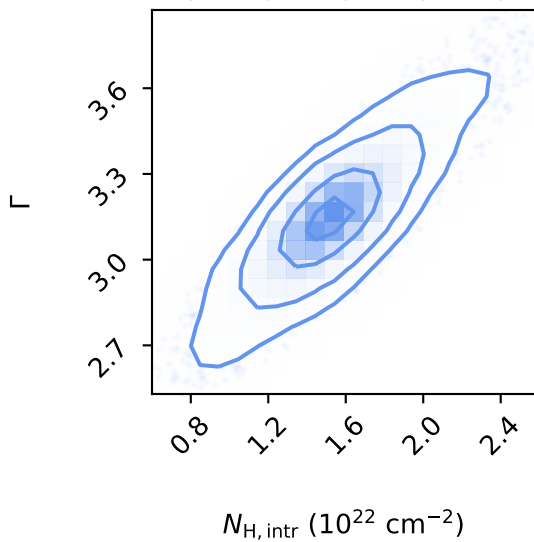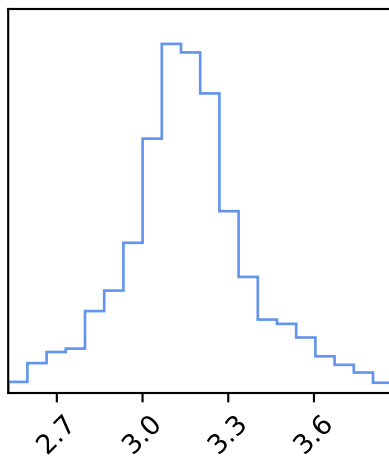

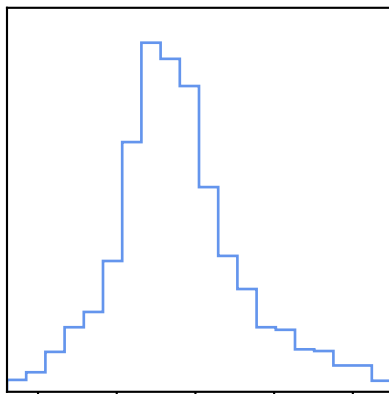

GRB171222A

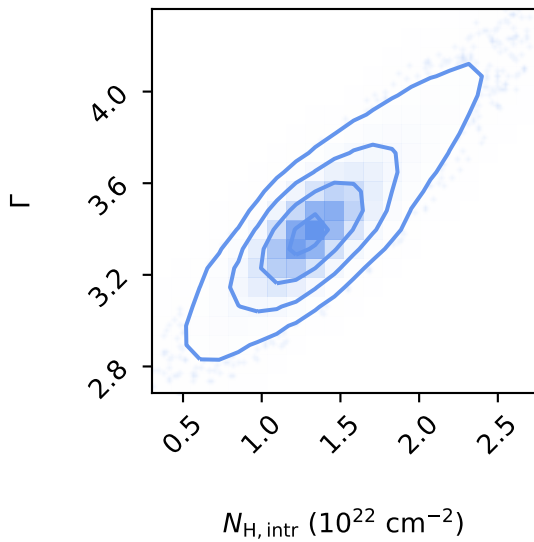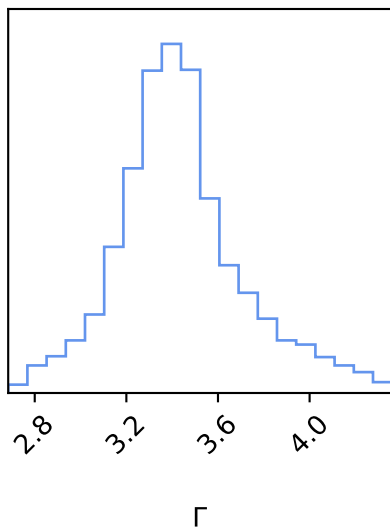

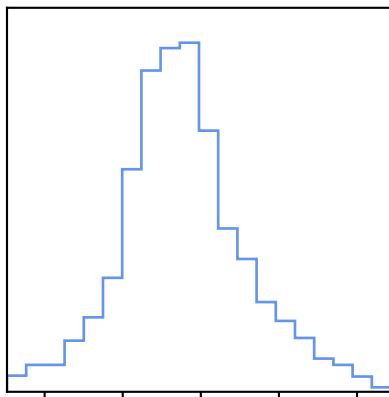

GRB171222A

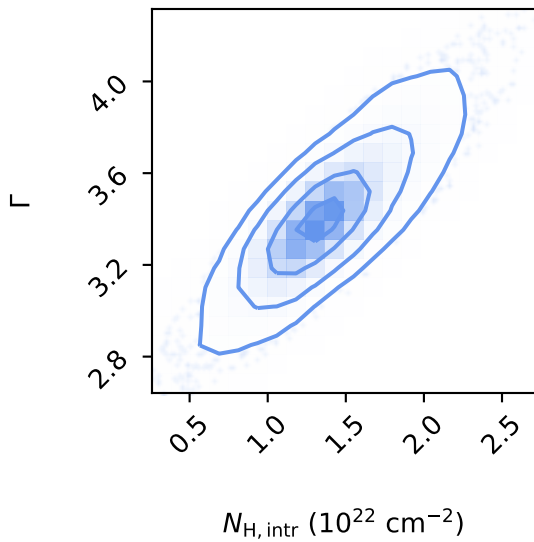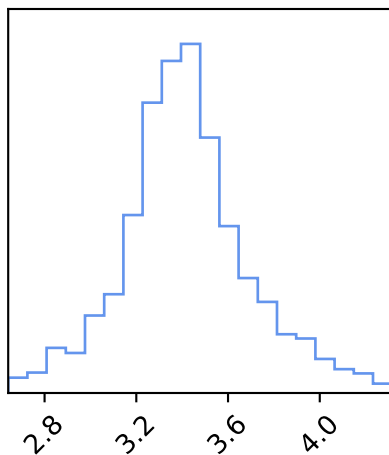



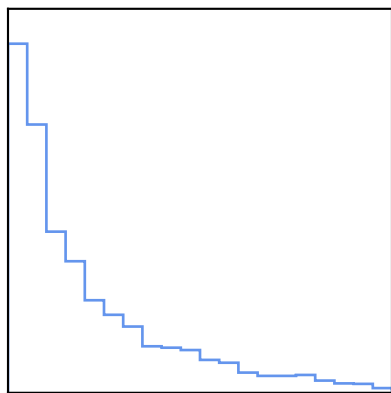

GRB171222A

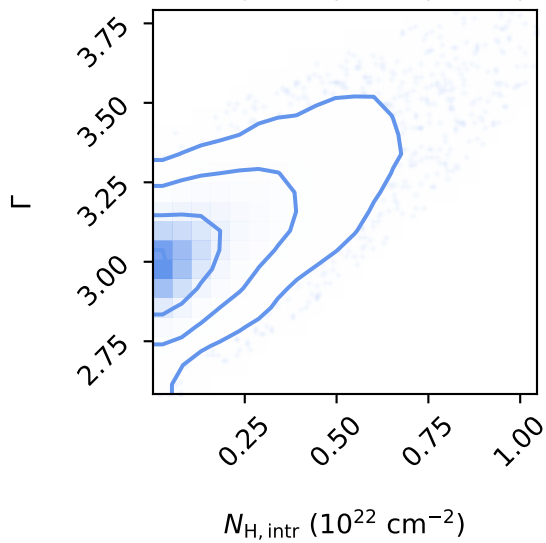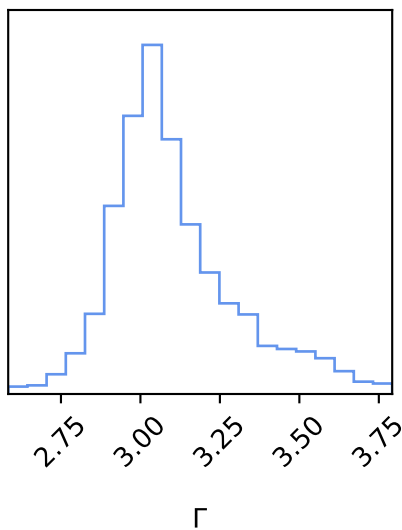

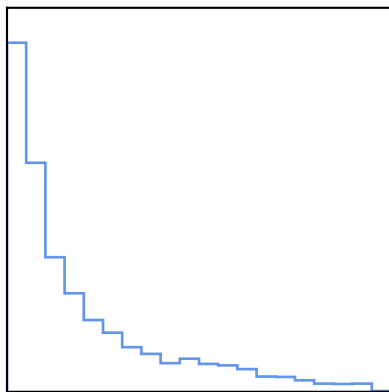

GRB171222A

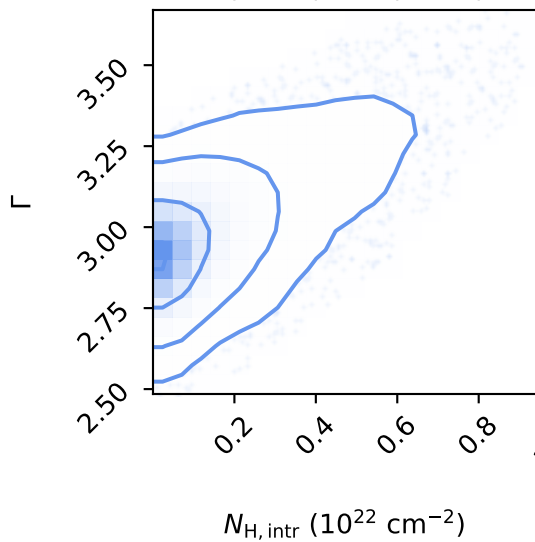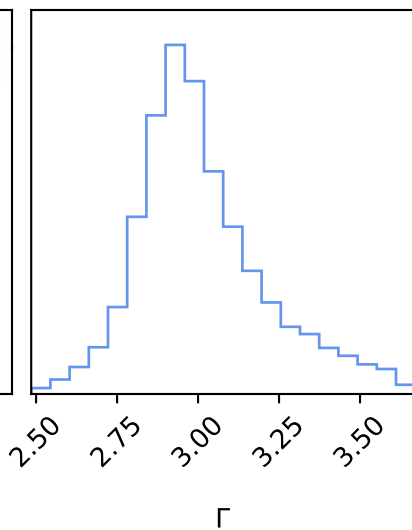

Supplement: Supplementary file 13 [file GRB171222A_cornerplot.pdf]
